# Supplementary material for: Unveiling Phonon Contributions to Thermal Transport and the Failure of the Wiedemann-Franz Law in Ruthenium and Tungsten Thin Films
Source: arXiv:2505.07613 source file (2025-05-12)
Supplement: Supplementary file 1 [file Supporting_Information.pdf]

# Supporting Information: Unveiling Phonon Contributions to Thermal Transport and the Failure of the Wiedemann-Franz Law in Ruthenium and Tungsten Thin Films

Md. Rafiqul Islam[1], Pravin Karna[2], Niraj Bhatt[2], Sandip Thakur[2], Helge Heinrich[3], Daniel M. Hirt[1], Saman Zare[1], Christopher Jezewski[4], Rinus T.P. Lee[5], Kandabara Tapily[5], John T.Gaskins[6], Colin D. Landon[7], Sean W. King[8], Ashutosh Giri[2], and Patrick E. Hopkins*[1,9,10]

[1]Department of Mechanical and Aerospace Engineering, University of Virginia, Charlottesville, Virginia 22904, USA
[2]Department of Mechanical Industrial and Systems Engineering, University of Rhode Island, Kingston, RI 02881, USA
[3]Nanoscale Materials Characterization Facility, University of Virginia, Charlottesville, Virginia 22904, USA
[4]Components Research, Intel Corporation, Hillsboro, Oregon 97124, USA
[5]TEL Technology Center, America, Albany NY 12203, USA
[6]Laser Thermal, Charlottesville, Virginia 22902, USA
[7]Logic Technology Development, Intel Corporation, Hillsboro, Oregon 97124, USA
[8]Supplier, Technology, and Industry Development, Intel Corporation, Hillsboro, Oregon 97124, USA
[9]Department of Materials Science and Engineering, University of Virginia, Charlottesville, Virginia 22904, USA
[10]Department of Physics, University of Virginia, Charlottesville, Virginia 22904, USA

# Contents

Section S1. Scanning transmission electron microscopy (STEM characterization of Ru and W films (Page 3)
Section S2. First principles-calculation to obtain the thermal conductivity and electron-phonon coupling factor of Ru and W films (Page 08)
Section S3: Methodology and lattice thermal conductivity results using machine-learned potential (Page 10)
Section 4: Spectral Energy Density (SED) Calculations (Page 13)
Section S5: TDTR thickness, sensitivity, uncertainty, and data analysis (Page 16)
Section S6: SSTR sensitivity, uncertainty, and data analysis (Page 22)
Section S7: Beam offset technique (Page 24)
Section S8. Details on two temperature model (TTM) and electron-phonon coupling factor determination (Page 25)
Section S9. Effective electron relaxation time determination with an infrared ellipsometer (Page 31)
Table S1: Table S1: The atomic fraction of oxygen and silicon from EDX analysis on as-deposited and annealed Ru films (page 5)
Table S2: Table S2: The atomic fraction of oxygen from EDX analysis on as-deposited tungsten films (page 7)
Table S3: The average roughness of Ru and W films (page 07)
Table S4. Parameters used in sensitivity analysis and the thermal model to determine the in-plane and cross-plane thermal conductivities of the Ru and W films (Page 21)
*Table S5: Comparison of SSTR, and TDTR measured in-plane thermal conductivities of Ru and W films (page 24)*
Table S6. Parameters utilized for the two-temperature model calculations in this work (Page 33)

## S1. Scanning transmission electron microscopy (STEM) characterization of Ru and W films

We use physical vapor deposition (PVD) to synthesize a series of Ru films with thicknesses ranging from 5 nm to 100 nm on 100 nm $SiO_2$/Si substrates. Similarly, we deposit W films with thicknesses between 3 nm and 101 nm on 3 nm Ta/100 nm $SiO_2$/Si substrates using the PVD technique. To study the role of experimental parameters on different properties, we synthesize W films through two distinct approaches: one focused on reducing resistivity (labeled as $W_R$) and the other on modifying grain size (assigned as $W_G$). We then characterize the microstructure, chemical composition, and crystallography of selected Ru and W films using scanning transmission electron microscopy (STEM).

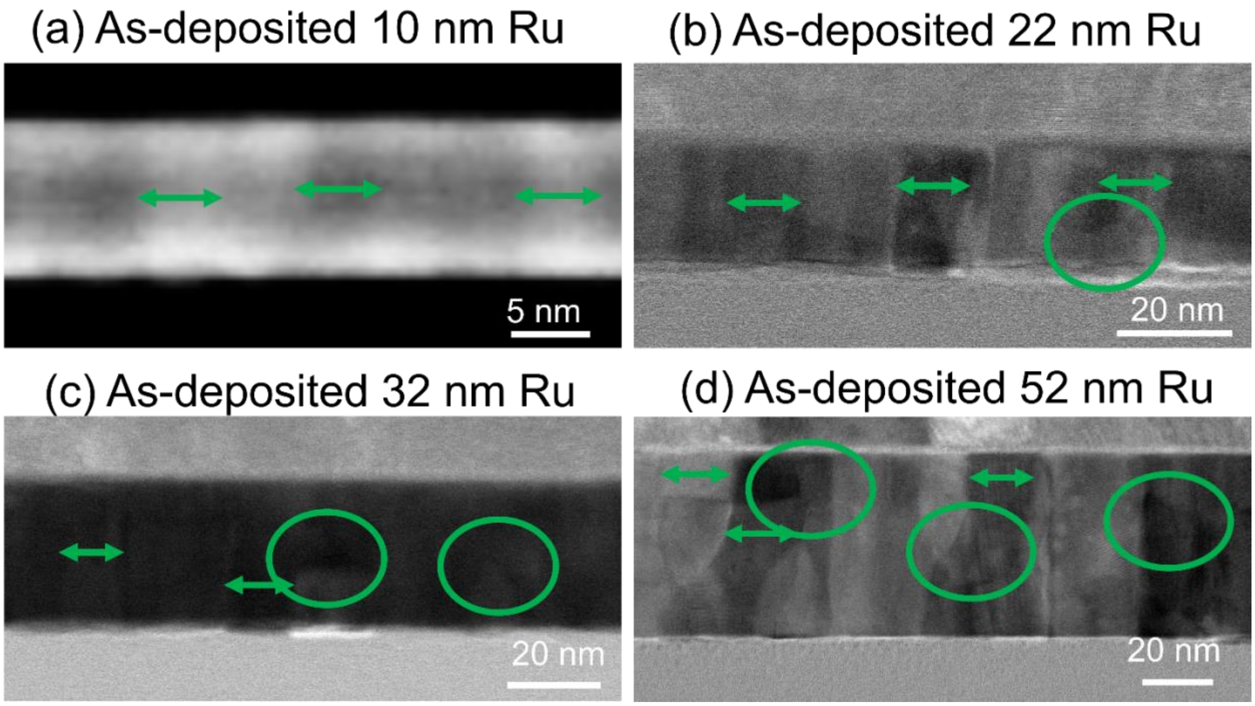


*Figure S1: STEM micrographs for PVD grown as-deposited (a) ~10 nm, (b) ~22 nm, (c) ~32 nm and (d) ~52 Ru films. The green arrows indicate grain size and green circle indicates the presence of irregular or equiaxed grains.*

Figure S1 illustrates the mixed grain morphology of as-deposited Ru films, where columnar grains are predominant, while some grains, highlighted by circles, display irregular or equiaxed shapes. Additionally, several grains transform from an equiaxed structure near the interface to a columnar form as they grow vertically. Our chemical composition analysis using STEM-EDX confirms that both as-deposited and annealed Ru do not contain significant impurities. Figure S3 and Table S1 show the presence of silicon in the EDX signal, which originates from the underlying 100 nm $SiO_2$ layer. Moreover, the Cu peak observed in the EDX spectrum arises from the Cu grid.

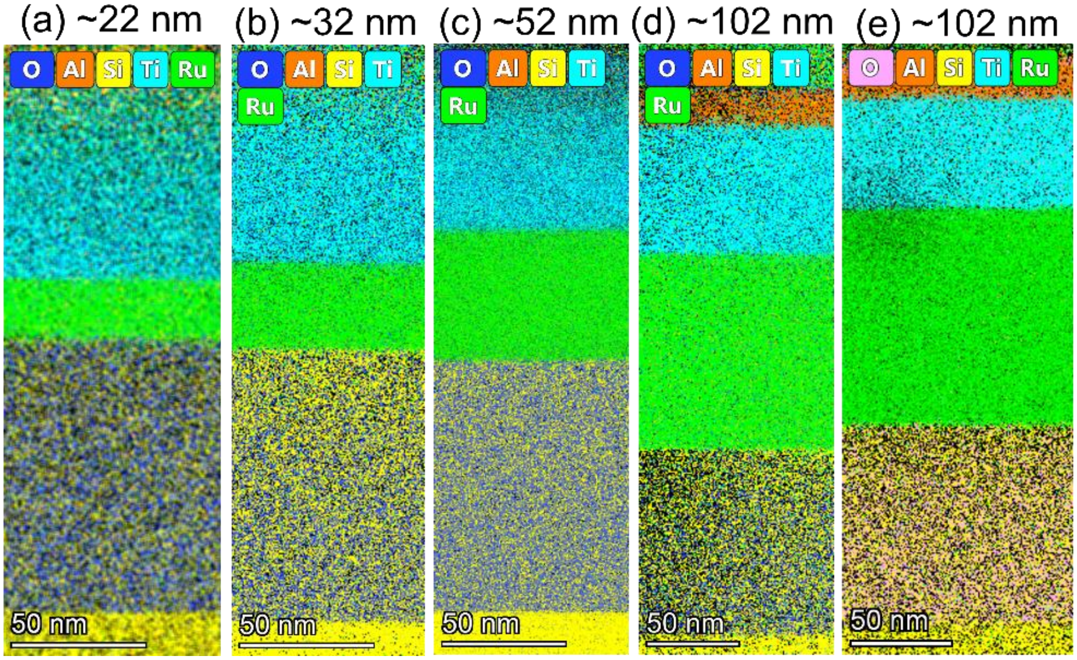


*Figure S2: STEM-EDX mapping for PVD grown as-deposited (a) ~22 nm, (b) ~322 nm, (c) ~32 nm, (d) ~52 Ru films and annealed (e) ~102 nm films. These films do not contain noticeable impurity.*

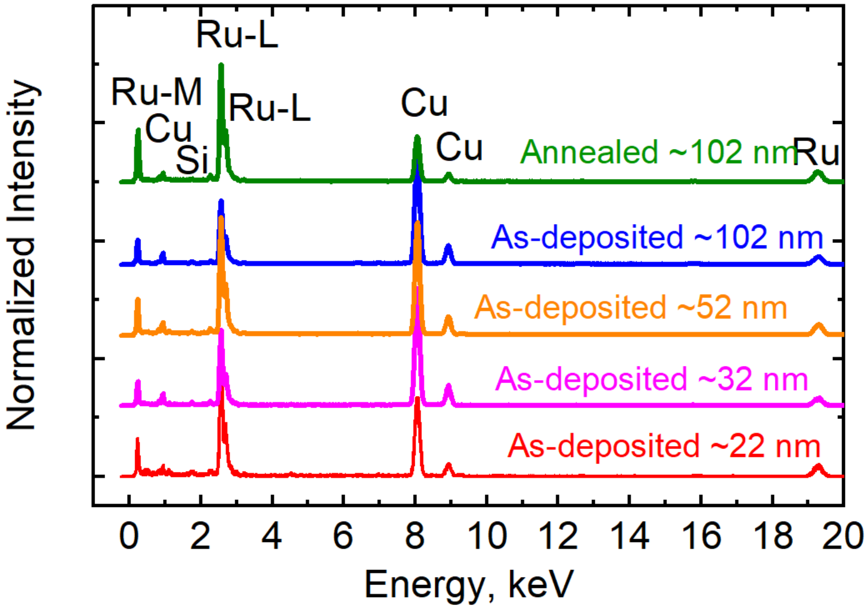

*Figure S3: STEM-EDX spectra for PVD grown ~22 nm, ~32 nm, ~52 nm, ~102nm as-deposited Ru films and ~102 nm annealed Ru films. Silicon in the EDX signal originates from the underlying 100 nm SiO2 layer.*

Table S1: The atomic fraction of oxygen and silicon from EDX analysis on as-deposited and annealed Ru films

| As-deposited Ru films, nm | Oxygen atomic fraction (%) | Silicon atomic fraction (%) | Annealed Ru films, nm | Oxygen atomic fraction (%) | Silicon atomic fraction (%) |
|---|---|---|---|---|---|
| ~22 | 0.0 | 3.9±0.02 | | | |
| ~32 | 0.0 | 3.1±0.03 | | | |
| ~52 | 0.0 | 2.4± 0.03 | | | |
| ~102 | 0.0 | 5.2±0.06 | ~102 | 2.2±0.01 | 0.9±0.03 |

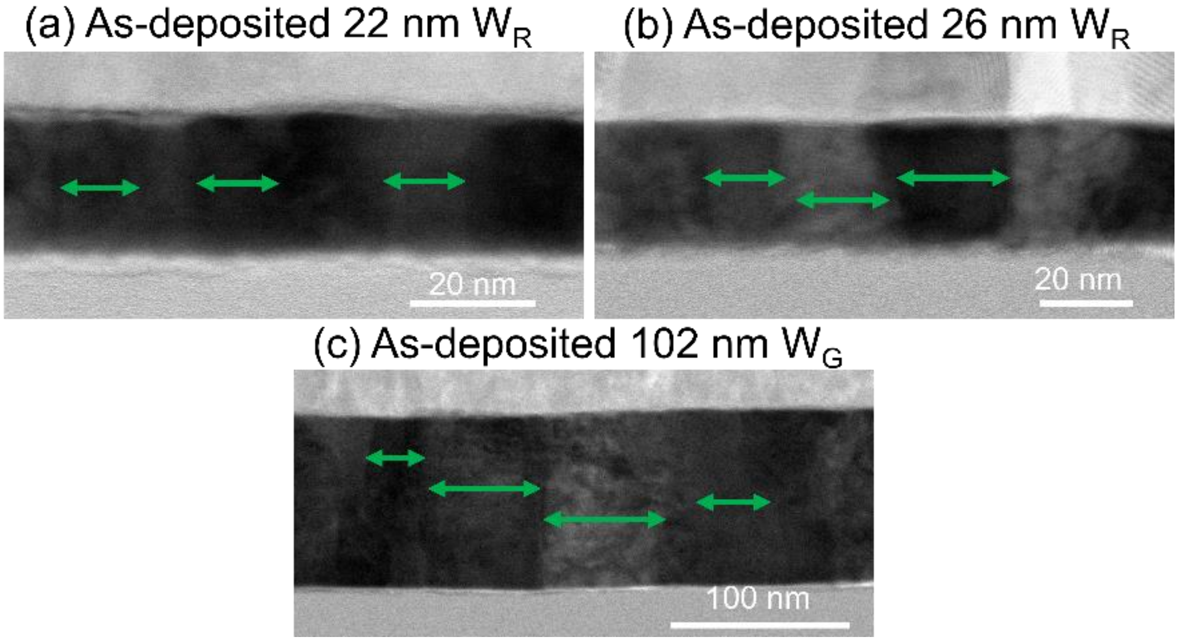


*Figure S4: STEM micrographs for PVD grown as-deposited (a) ~22 nm $W_R$, (b) ~32 nm $W_R$ and (c) ~102 nm $W_G$ films. The green arrows indicate the grain size, which increases with thickness. The grains in the tungsten films are columnar.*

We also analyze the grain size and thickness of tungsten films ($W_R$ and $W_G$). As shown in Figure S4, the grain sizes of $W_R$ films remain within a similar range. However, the grain size of the ~102 nm film is notably larger compared to the thinner films. The chemical composition of these films is further verified through STEM-EDX analysis, as presented in Figures S5 and S6 and summarized in Table S2. Oxygen is detected in the films, primarily originating from the transfer process of the prepared thin samples from the FIB to the STEM chamber. Additionally, a 1–2 nm layer of native tungsten oxide may have formed on the W surface. The presence of carbon (C) and

molybdenum (Mo) in the EDX spectrum is attributed to the FIB-SEM and STEM characterization processes. Carbon is intentionally deposited on W films to achieve a clean surface, facilitating the identification of the top surface layer in FIB-SEM and STEM imaging. The Mo peak observed in the EDX spectrum arises from the Mo grid. In summary, EDX analysis confirms that the Ru and W films are free from general impurities, although W films contain a small amount of oxygen

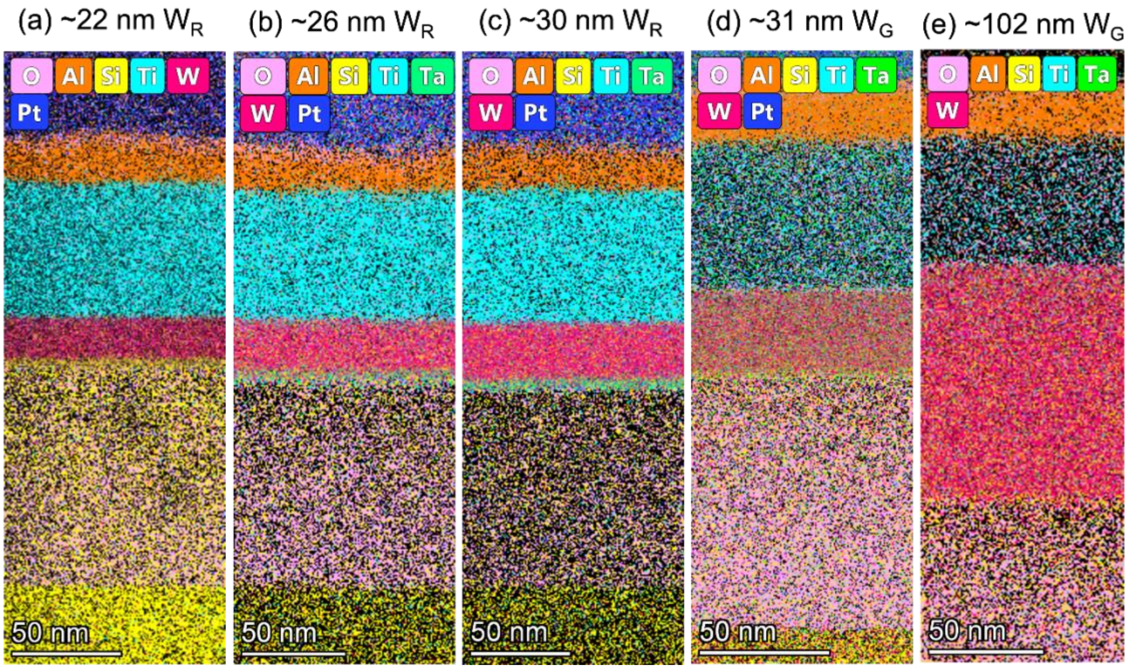


*Figure S5: STEM-EDX mapping for PVD grown as-deposited (a) ~22 nm $W_R$, (b) ~26 nm $W_R$, (c) ~30 nm $W_R$, (d) ~ 31$W_G$ and (e) ~102 nm $W_G$ films. These films do not contain noticeable impurity.*

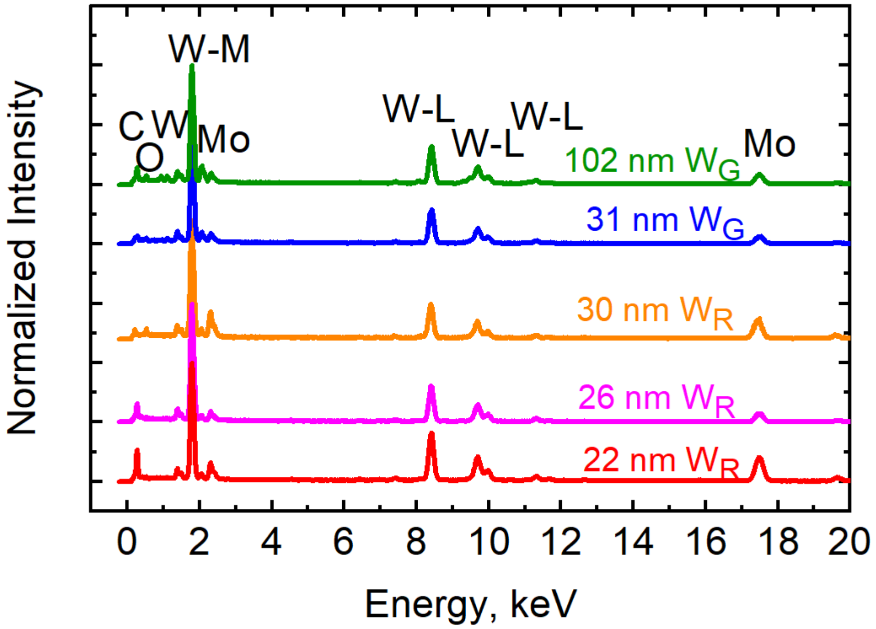

*Figure S6: STEM-EDX spectra for PVD grown as-deposited ~22 nm $W_R$, ~26 nm $W_R$, ~30 nm $W_R$, ~ 31 nm $W_G$ and ~102 nm $W_G$ films. The detected oxygen originates from the transfer process of the prepared thin samples from the FIB to the STEM chamber. Additionally, a 1–2 nm layer of native tungsten oxide may have formed on the W surface. The detection of carbon (C) and molybdenum (Mo) in the EDX spectrum is associated with the FIB-SEM and TEM characterization process.*

Table S2: The atomic fraction of oxygen from EDX analysis on as-deposited tungsten films

| As-deposited $W_R$ films, nm | Oxygen atomic fraction (%) | As-deposited $W_G$ films, nm | Oxygen atomic fraction (%) |
|---|---|---|---|
| ~22 | 4.1±0.04 | | |
| ~26 | 6.3±0.21 | | |
| ~30 | 4.7±0.07 | ~31 | 4.4±0.21 |
| | | ~102 | 5.7±0.27 |

We measure the surface roughness of Ru and W films using a Zygo NewView 7300 interference microscope, with additional measurement details provided elsewhere.[1] Briefly, we employ three-dimensional white-light interferometry, a non-contact profilometry technique. The microscope features a 20× Mirau interference objective, a 150 µm piezoelectric vertical turret, a digital black-and-white camera (640 × 480 pixels), and Zygo's proprietary image analysis software. The field of view is 350 × 260 µm, and the system provides an axial resolution of ~0.1 nm with a repeatability of <0.3 nm. The average roughness of the Ru and W films remains nearly identical across thicknesses and is very low (~≤ 1 nm), as summarized in Table S3.

Table S3: The average roughness of Ru and W films

| Ru film, nm | Average roughness, nm | W films, nm | Average roughness, nm |
|---|---|---|---|
| As-deposited ~52 nm | 0.98±0.14 | As-deposited 26 nm $W_R$ | 0.58±0.02 |
| As-deposited ~102 nm | 0.67±0.05 | As-deposited 30 nm $W_R$ | 0.62±0.07 |
| Annealed ~52 nm | 0.89±0.12 | As-deposited 50 nm $W_G$ | 0.41±0.05 |
| Annealed ~102 nm | 1.02±0.09 | As-deposited 101 nm $W_G$ | 0.46±0.01 |

We also determine the thickness of the Al and Ti transducers using STEM, as shown in Figure S07. We utilize these transducers to perform the steady-state and time-domain thermoreflectance measurements.

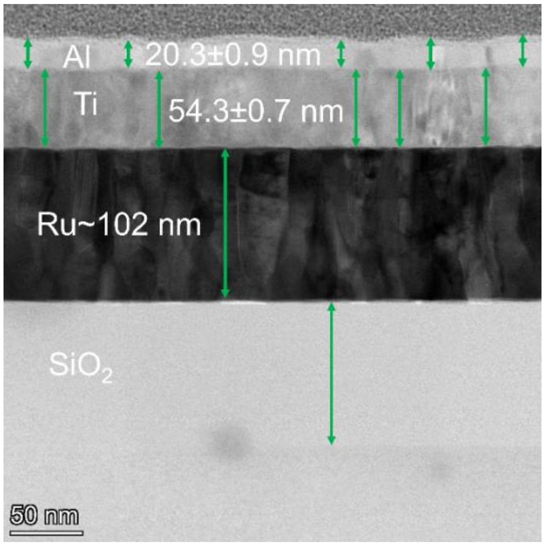


*Figure S07: STEM image of Al/ Ti coated 102 nm annealed Ru film.*

**S2: First principles-calculation to obtain the thermal conductivity and electron-phonon coupling factor of Ru and W films**

We obtain the electron-thermal conductivity and electron-phonon coupling factor of Ru and W films through First principles calculations. The details of our calculations can be found in our previous work. [2,3] The interpolation of the electron-phonon matrix elements, phonon modes, and band energies from an initial coarse grid (10 × 10 × 10 and 5 × 5 × 5) to a uniform fine grid (80 × 80 × 80 and 35 × 35 × 35) for electron and phonon wave vector grids is achieved using Electron phonon Wannier (EPW) package which is incorporated within the Quantum Espresso software. We use norm-conserving pseudopotential for both Ru and W which is obtained from the PS Library.

We calculate the Eliashberg spectral function $\alpha^2F(\omega)$ at room temperature for Ru and W using density functional perturbation theory calculation. A corresponding mass enhancement parameter, $\lambda$, is also calculated which is 0.52 and 0.29 for Ru and W respectively. The calculated values of $\lambda$ matches well with prior literature.[4] We calculate the average mean free path of Ru and W from the calculated electron-phonon scattering rates which are ~ 15.5 nm for W and ~6 nm for Ru. The calculated Fermi velocity as obtained from the Fermi surface is ~$6\times10^5$ m $s^{-1}$ for Ru and ~$9.4\times10^5$ m $s^{-1}$ for W.

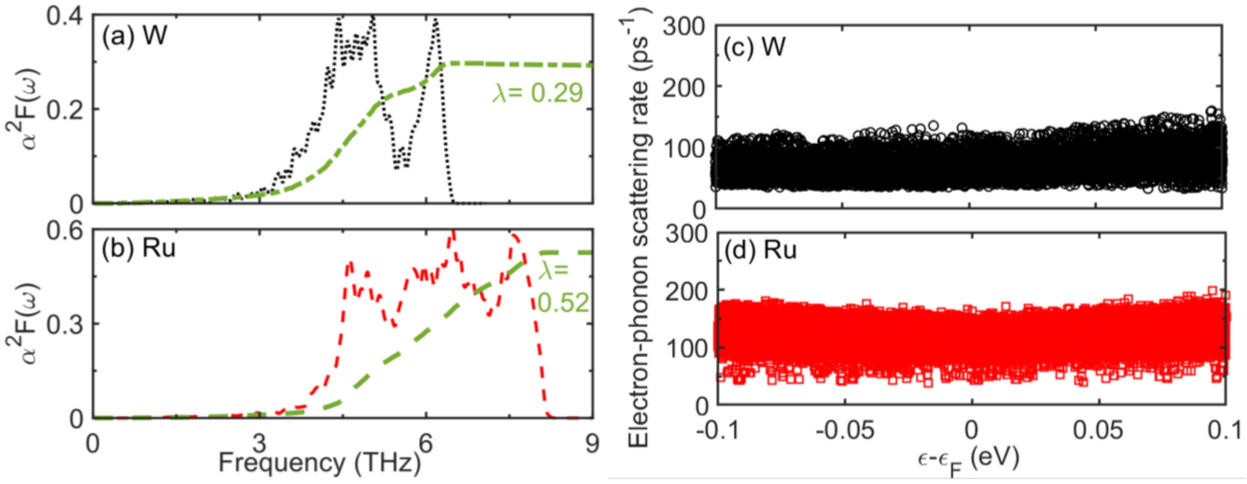


*Figure S08: Calculated Elishberg spectral function for (a) W and (b) Ru. The dashed lines represent the corresponding mass enhancement parameter. Calculated electron-phonon scattering rates for (c) W and (d) Ru.*

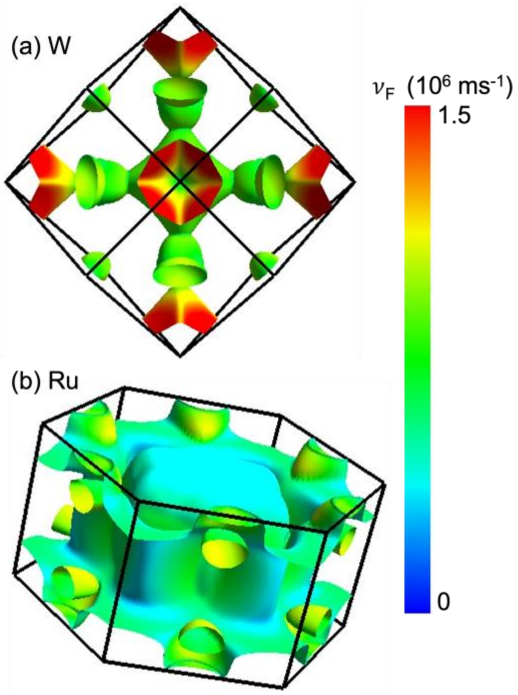


*Figure S09: Calculated Fermi surface for (a) W and (b) Ru. The color on the Fermi surfaces are representative of the Fermi velocities of the electrons on the Fermi surface.*

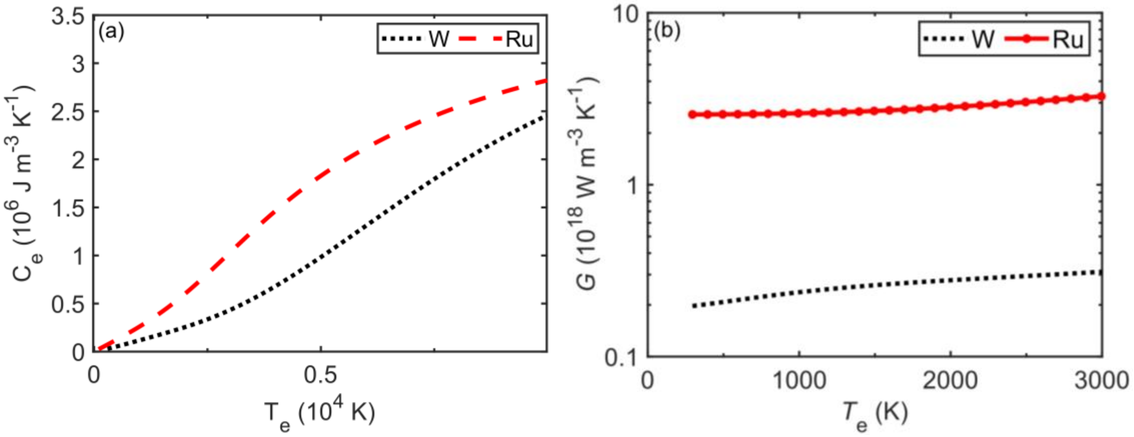


Figure S10: (a) Electronic emperature dependent electronic heat capacity for W and Ru. (b) Electronic temperature dependent volumetric electron-phonon coupling factor for W and Ru.

We calculate the electronic heat capacity of the metals using,

$$C_{\mathrm{e}}(T_{\mathrm{e}}) = \int_{-\infty}^{\infty} \frac{\partial f(\varepsilon,\mu,T_{\mathrm{e}})}{\partial T_{\mathrm{e}}} g(\varepsilon)\varepsilon d\varepsilon, \qquad \text{(S01)}$$

where $g(\varepsilon)$ denotes the eDOS at the energy level $\varepsilon$, $\mu$ is the chemical potential at $T_{\mathrm{e}}$, and $f(\varepsilon,\ \mu,$ $T_{\mathrm{e}})$ denotes fermi distribution function, defined as $f(\varepsilon,\mu,T_{\mathrm{e}}) = \{\exp\,[(\varepsilon-\mu)/k_{\mathrm{B}}T_{\mathrm{e}}]\ + 1\}^{-1}$.

We also calculate the volumetric rate of e-p coupling, which is given as,

$$G = \pi\hbar k_B \lambda\langle\omega^2\rangle \int_0^{\infty} \frac{(D(\varepsilon))^2}{D(\varepsilon_F)} \left[-\frac{\partial f}{\partial \varepsilon}\right] d\varepsilon, \quad \text{(S02)}$$

where $\langle\omega^2\rangle$ represents the second moment of the phonon spectrum and $D(\varepsilon)$ is the eDOS. At room temperature, the calculated $G$ is ~$2\times10^{17}$ W m$^{-3}$ K$^{-1}$ for W and ~$2.5\times10^{18}$ W m$^{-3}$ K$^{-1}$ for Ru which matches closely with previous calculations.[4] From the calculated $C_{\mathrm{e}}$, $v_{\mathrm{F}}$ and $\Lambda$, we calculate the thermal conductivity as detailed in our previous works.[2–4] The calculated electronic thermal conductivity for W and Ru is 135 W m$^{-1}$ K$^{-1}$ and 97 W m$^{-1}$ K$^{-1}$ , respectively.

We introduce the effect of boundary scattering on the total scattering rate of the electrons as,[5]

$$\frac{1}{\tau_{tot}} = \frac{v_F}{\Lambda} + \frac{v_F}{d} + \frac{v_F}{D} + \frac{v_F}{\Lambda_{defect}} \qquad \text{(S03)}$$

$\tau_{tot}$ represents the total scattering time which includes electron-phonon scattering rate as well as the boundary scattering of the electrons. In this formulation, d denotes the thickness of the thin film, D is the grain-size, $\Lambda_{defect} = \frac{a}{\sqrt{c}}$ represents the effective mean free path associated with point defect scattering, where a is the lattice constant and c is the defect concentration.[6] In this work, we assume a point defect concentration of 0.2% in both Ru and W thin films.[7,8] Electron–electron scattering is neglected, as electron–phonon interactions dominate at room temperature.

**S3: Methodology and lattice thermal conductivity results using machine-learned potential**

I. Training Data:

We develop a precise interatomic potential using a diverse training dataset produced by ab-initio molecular dynamics. During simulations at finite temperature, snapshots of the MD trajectory are taken, encompassing a range from various pressures at ambient temperatures. These snapshots offered atomic coordinates, forces, energies, and cell parameters, enabling thorough exploration

of the configurational space. The diversity of the data is essential as the accuracy of the machine-learned potential heavily depends on the quality and diversity of the training data. The Quantum Espresso package is used for all ab-initio MD simulations.[9] The exchange-correlation interactions are described using the PBE functional. The plane wave expansion uses an energy cut-off of ~ 60 Ry, while the self-consistent field energy convergence is set to $10^{-6}$ a.u. The Monkhorst-Pack mesh samples the Brillouin zone over a 4×4×4 grid. To accommodate the partial occupancy of electrons, we employ Fermi-Dirac smearing, with a smearing width of 0.02 Ry for Brillouin-zone integration in Ru. The cell parameters are allowed to relax in all ab-initio MD simulations, utilizing the isobaric-isothermal setup. We maintain each simulation at zero pressure using the Parrinello-Rahman barostat,[10] while temperature is kept constant through the rescaling technique. A time step of 2 fs and the Verlet algorithm are utilized in all DFT-MD simulations. The training dataset includes snapshots of the trajectory from isothermal-isobaric simulations at ambient temperature. First, a 2x2x2 supercell with a hexagonal close-packed (hcp) lattice containing 16 atoms is relaxed at 0 bar, and the equilibrium lattice constant is determined. The equilibrium lattice constant is then uniformly compressed and expanded, and the atoms are equally perturbed in random directions to conduct subsequent isothermal-isobaric simulations at ambient temperature. The equilibrium lattice parameters are compressed and expanded by percentages ranging from ±0.5% to ±4%. Random atomic perturbations of up to 0.04 Å are applied. We conduct a 2 ps simulation for each perturbed configuration, resulting in 5, 000 data frames generated by ab-initio simulations. A set of 1, 000 data frames, not included in the training dataset, is used as a validation dataset to evaluate the model's accuracy.

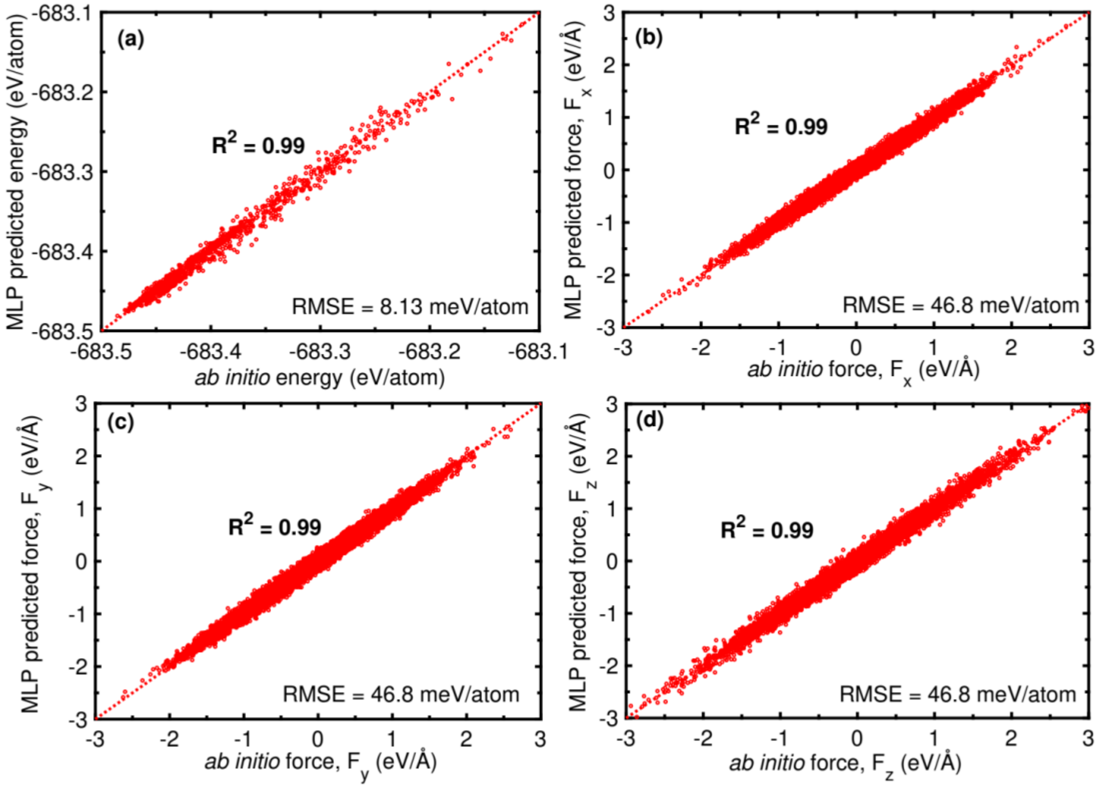


Figure S11: Validation plots comparing (a) energies and (b-d) forces from our MLP and ab initio MD for ruthenium at ambient temperature. The low RMSE as well as R-squared values close to

unity revealed perfect x=y agreement of MLP-predicted vs ab initio energies and forces indicate the accuracy of our MLP.

## II. Training procedure

We accurately map the energy space of an atom's position using the deep learning framework DEEPMD to create a DeepPot-SE neural model through dataset training. We employ DEEPMD integrated with the popular Tensorflow[11] deep learning framework for training and testing the machine-learned interatomic potential, as well as the widely used molecular dynamics package LAMMPS [12] for MD simulations. A cutoff radius of 6Å is established, and the descriptors decay from 0.5Å to 6Å to eliminate the discontinuity introduced by the cutoff. The neural architecture comprises two neural networks: one to convert atomic coordinates to descriptors and the other to map descriptors to their corresponding atomic energies. The former network is referred to as the embedding network, while the latter is known as the fitting network. The embedding network consists of three hidden layers with sizes of (25, 50, 100) following a Res-Net-like architecture. [13] The fitting network comprises three hidden layers, each with 240 neurons. Adam stochastic gradient descent approach is utilized for cost function optimization. The learning rate varies from $10^{-3}$to $10^{-8}$ with an exponential decay over 2, 000, 000 steps. The pre-factors of energies and forces are set as $P_e^{start}$ = 0.01, $P_f^{start}$=1, 000, $P_e^{limit}$==1, and $P_f^{limit}$= 1, respectively.

We utilize a test dataset of 1000 frames to assess the trained potential's accuracy. The test indicated an energy accuracy of $8.13\times10^{-3}$ eV/atom and a force accuracy of $46.87\times10^{-3}$ eV/Å , demonstrating the accuracy of the ML Potential as shown in Figure S11. We carry out all MD simulations using the large-scale atomic/molecular massively parallel simulator (LAMMPS) and the DEEPMD package. A timestep of 1.0 fs is utilized, and the velocity-verlet algorithm is implemented. Temperature and pressure is controlled using the Nose-Hoover thermostat and barostat, with damping parameters set at 0.1 ps and 1 ps for the thermostat and barostat, respectively. We apply periodic boundary conditions in all three directions.

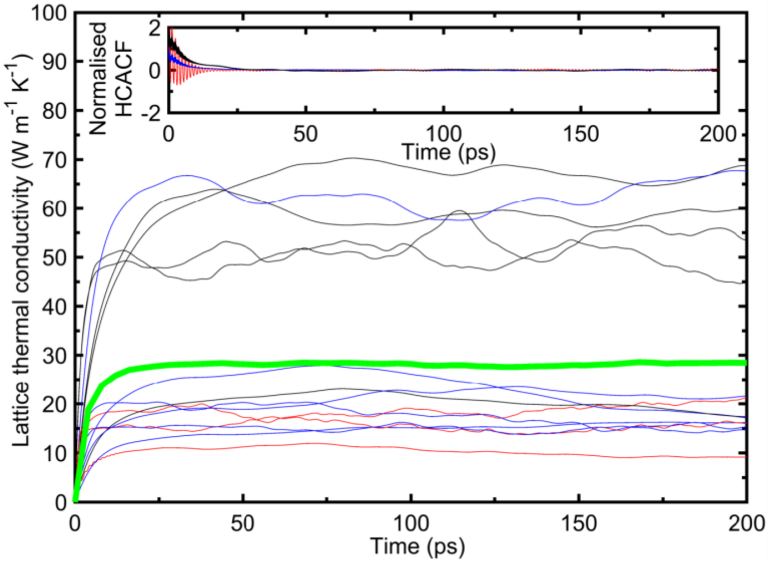


Figure S12. Green-Kubo predicted thermal conductivities for average five different runs as a function of the integration time for ruthenium at ambient conditions. The thick green lines denote

the average predicted thermal conductivities at room temperature. We average out the thermal conductivity by taking mean thermal conductivity from 50 ps to 200 ps. (inset) A fully decayed normalized heat current autocorrelation function (HCACF) as a function of the integration time

III. Calculating phonon thermal conductivity

We determine the phonon thermal conductivity of Ru using the Machine-learned potential and the EMD method based on the Green-Kubo formula. The lattice thermal conductivity associated with the heat current autocorrelation function (HCACF) can be expressed as

$$\kappa = \frac{1}{VK_bT^2}\int_0^{\infty} < J_{x,y,z}(0)J_{x,y,z}(t) > dt \qquad \text{(S04)}$$

where $K_b$ ,T ,V and t are the Boltzmann constant, temperature, volume, and time respectively, and $\langle J_{x,\ y,\ z}(0)\ J_{x,y,z}(t)\rangle$ is the heat current auto-correlation (HCACF) component along x,yor z-directions.

First, the lattice undergoes minimization using the conjugate gradient approach, followed by relaxation under the NPT ensemble for 50 ps at a target temperature and pressure of 0 bar. Subsequently, the system undergoes relaxation under the NVT ensemble for 50 ps. Lastly, the system is relaxed under the NVE ensemble for 10 ns, and data on heat current is collected to calculate the phonon thermal conductivity using the equation mentioned above. For calculating the lattice thermal conductivity for Ru at ambient, we use the well-known green-kubo formalism. The total correlation time period ranging from 50 ps to 200 ps is used to achieve converged heat current autocorrelation function (HCACF) for all our simulations. We use a sampling interval of 10 fs while collecting the data to calculate the HCACF at ambient temperature. Finally, the heat current autocorrelation function is integrated to get the converged thermal conductivity for Ru. We perform ~5 independent simulations at room temperature with different initial conditions as shown in Figure S12. The phonon thermal conductivity reported is estimated by taking the mean value of all the simulations. We obtain a lattice thermal thermal conductivity of 27.4 ±3 $Wm^{-1}K^{-1}$ at room temperature using our MLP. The uncertainties quantified by standard deviation range less than 12% in all our simulations.

**S4: Spectral Energy Density (SED) Calculations**

We perform MD simulations using the SED formalism to analyze the atomic-scale dynamics of the material. In this approach, we apply a Fourier transform to the atomic velocities to calculate the average kinetic energy per unit cell as a function of wave vector (**q**) and frequency (ω), which is expressed as,[14,15]

$$\Phi(\mathbf{q},\omega) = \frac{1}{4\pi\tau N_T}\sum_{\alpha}^{3}\sum_{b}^{B} m_b \left|\int_0^{\tau}\sum_{n_{x,y,z}}^{N_T} \dot{u}_{\alpha}\binom{n_{x,y,z}}{b};t\right) \times exp\left[i\mathbf{q}\cdot\mathbf{r}\binom{n_{x,y,z}}{0} - i\omega t\right] dt\right|^2 \qquad \text{(S05)}$$

Here $\tau$ is the total simulation time, α represents the Cartesian direction, and $n_{x,y,z}$ denotes a unit cell. $N_T$ is the total number of unit cells in the crystal, $b$ represents the atomic index in a given unit cell, $B$ is the atomic number in the unit cell, and $m_b$ is the mass of atom $b$ in the unit cell. $\dot{u}_\alpha$ denotes the velocity in the α-direction at time $t$, and **r** represents the equilibrium position of each unit cell.

For the SED calculations, we construct a computational domain by replicating the unit cell to form a supercell of dimensions of $4 \times 100 \times 4$. The system is first equilibrated using the Nos\'e-Hoover thermostat and barostat (i.e. the NPT ensemble)[16] for 2 ns with a timestep of 0.5 fs, maintaining a constant number of particles, pressure, and temperature at 0 bar. This is followed by an additional 2 ns equilibration under the NVT ensemble, where the volume and temperature remain fixed. Finally, MD simulations are conducted in the microcanonical ensemble (NVE) for 1.5 ns with a 0.5 fs timestep, during which atomic configurations are recorded for SED calculations.

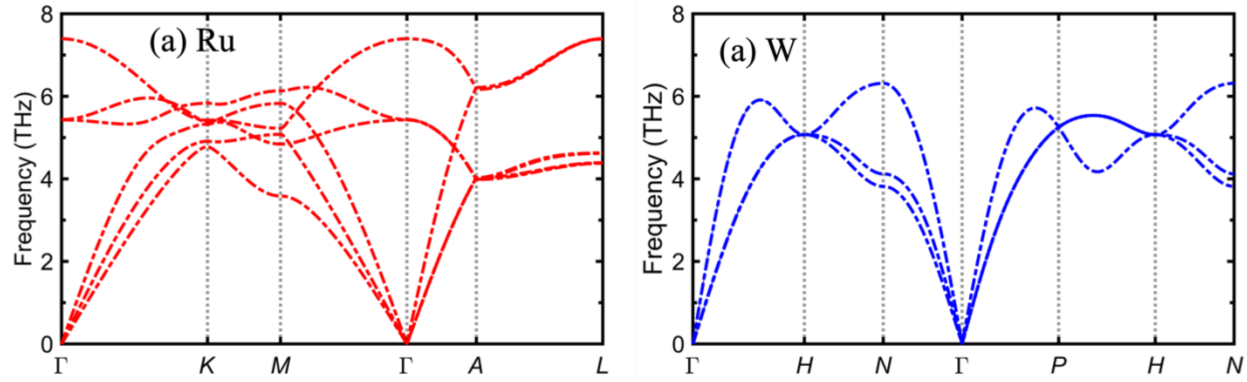


*Figure S13: Phonon dispersion curves for (a) Ru (red) and (b) W (blue) along high-symmetry paths in their respective Brillouin zones. The frequency of vibrational modes is plotted as a function of wave vector, showing characteristic dispersion behavior. The presence of zero-frequency modes at the Γ point indicates acoustic phonon branches, while the higher-frequency branches correspond to optical phonon modes.*

Based on the phonon dispersion curves (Figure S13), Ru exhibits both acoustic and optical branches, while W primarily shows acoustic branches without distinct optical modes. In Ru, the optical branches appear above 4 THz, indicating higher-frequency lattice vibrations due to interatomic interactions. In contrast, W's dispersion curves remain within the acoustic regime, suggesting a lack of optical phonon modes, which could be attributed to its crystal structure and bonding characteristics

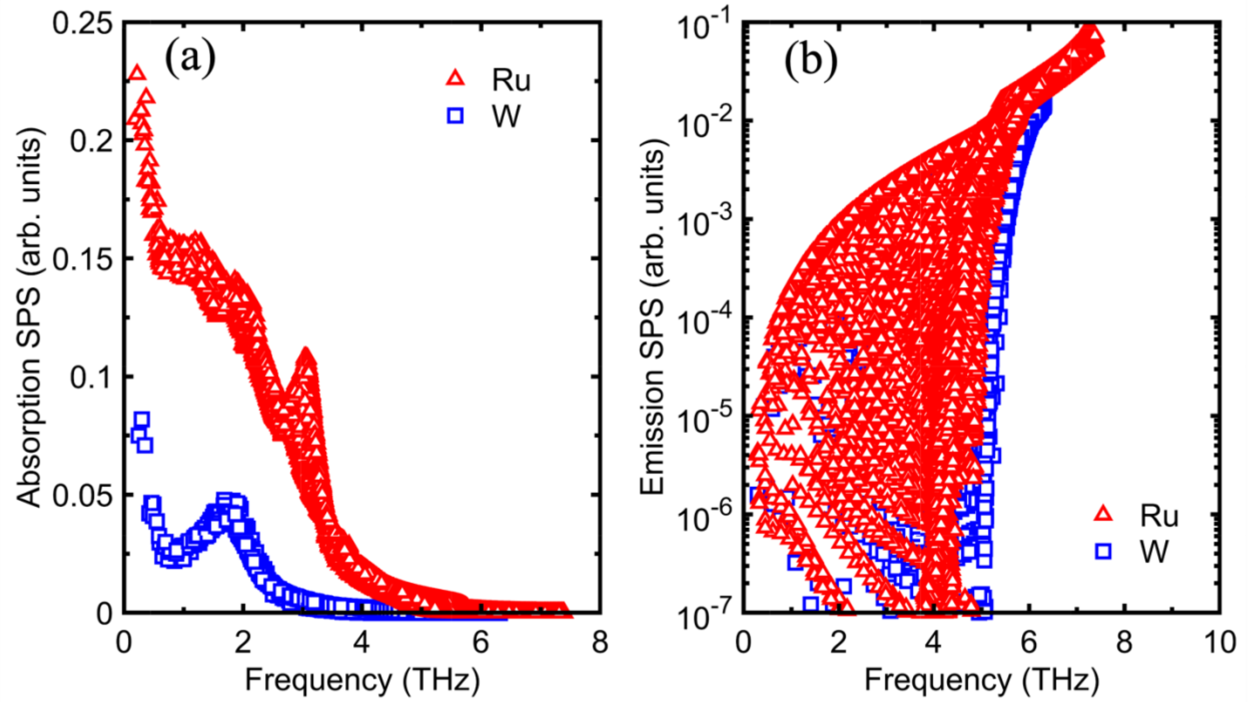


Figure S14: Comparison of the (a) absorption, and (b) emission scattering phase space

Ru exhibits a high absorption SPS at low frequencies, which generally indicates that Ru supports a greater number of phonon-phonon absorption events. This enhances momentum-conserving scattering (Normal processes), contributing to phonon thermalization without necessarily limiting heat conduction[17]. In contrast, a high emission SPS in Ru at certain frequencies reflects a large number of allowed phonon decay processes, which often enhance Umklapp (U) scattering. These resistive processes lead to shorter phonon lifetimes and reduced phonon thermal conductivity. This behavior is evident in Figure S15.

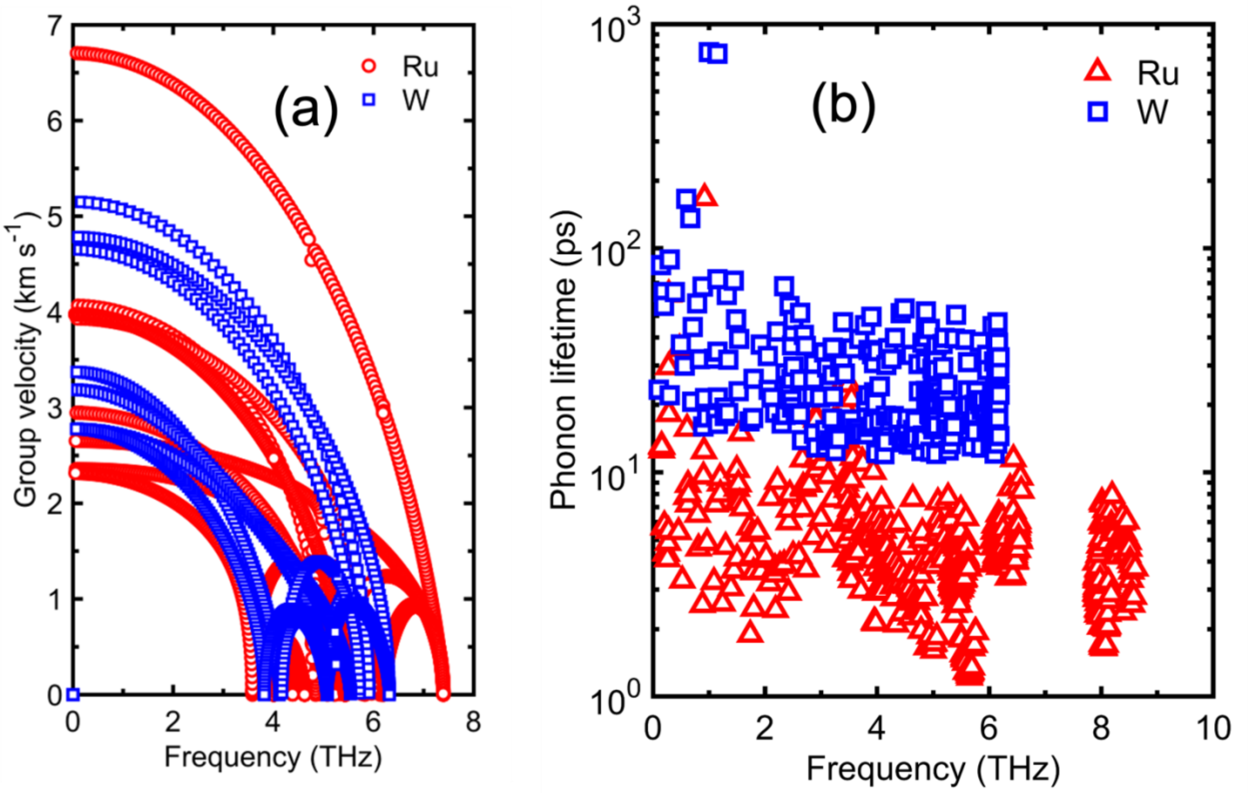


*Figure S15: The group velocity and phonon lifetime of Ru and W.*

**S5: TDTR thickness, sensitivity, uncertainty, and data analysis**

To support steady-state thermoreflectance measured in-plane thermal conductivity, we determine various thermophysical properties using time-domain thermoreflectance (TDTR), with details provided elsewhere[1,18]. A Ti:sapphire laser (~808 nm, 80 MHz, Spectra Physics Tsunami) generates a pump and probe beam, with the pump beam modulated via an electro-optic modulator (EOM) to induce a periodic temperature rise, altering the sample's reflectivity. The probe beam detects reflectivity changes using a balanced photodetector and lock-in amplifier. The schemetic for the TDTR set up is shown in Figure S16. To determine the pump and probe beam spot size at 20× magnification, we use an Al-coated fused silica calibration sample (Corning HPFS 7980, 1.36 $Wm^{-1}K^{-1}$). By fitting the known thermal conductivity in our thermal model, we obtain an effective beam radius of ~2.15 µm. Assuming identical pump and probe beam sizes, we verify the spot size by measuring the thermal conductivity of a sapphire calibration sample

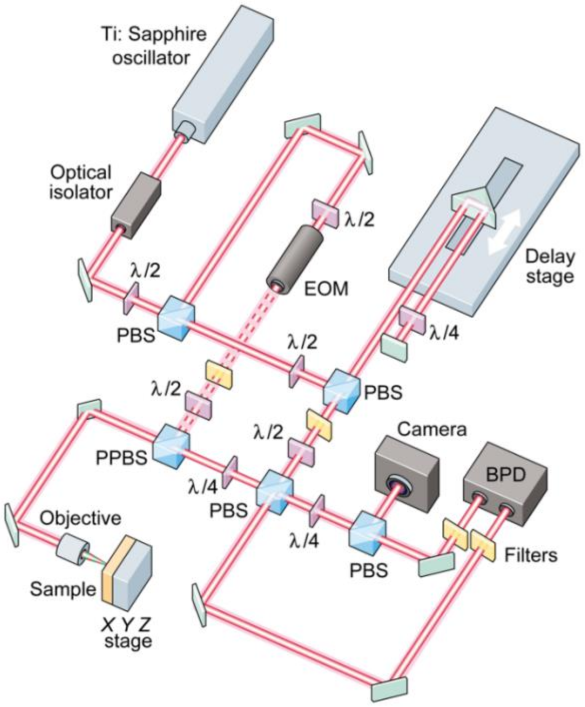


*Figure S16: Schematic of the TDTR experimental setup configuration*

We evaluate the sensitivity of TDTR measurements to the cross-plane and in-plane thermal conductivities of 102 nm Ru and W films, following the methodology described in our previous work on Cu films.[1] Briefly, a 20 nm Al/60 nm Ti transducer is used to ensure optical opacity and enhance heat spreading within the Ru and W layers relative to the transducer. The sensitivity to cross-plane and in-plane thermal conductivities is calculated at two modulation frequencies and a tightly focused spot size. Notably, a larger spot size results in shallower thermal penetration depth, thereby reducing sensitivity to thermal conductivities.[1,19] These calculations incorporate the thermophysical properties of each layer as listed in Table S4. As shown in Figure S17b and S17d, the sensitivity to the in-plane thermal conductivity of 102 nm Ru and W is higher at 1.2 MHz and a 2.15 μm effective radius, attributed to the greater thermal penetration depth. In contrast, the sensitivity to cross-plane thermal conductivity is comparable at 1.2 MHz and 8.4 MHz but remains lower than the in-plane sensitivity. To minimize the interdependence on in-plane thermal conductivity, we measure the cross-plane component at 8.4 MHz. However, TDTR measurements are limited to cross-plane and in-plane thermal conductivities for 102 nm Ru and W films and lose sensitivity for films with thickness ≤ 50 nm. Note, due to uncertainties in our calculations, we are unable to accurately measure the in-plane thermal conductivity of as-deposited ~102 nm Ru. We can measure the in-plane thermal conductivity of annealed ~102 nm Ru film with TDTR. Moreover, TDTR exhibits higher sensitivity to the thermal conductivity of $SiO_2$ and Si compared to Ru and W. To ensure accurate fitting of the experimental data, we incorporate accepted literature values for $SiO_2$ and Si[20–24] in our thermal model.

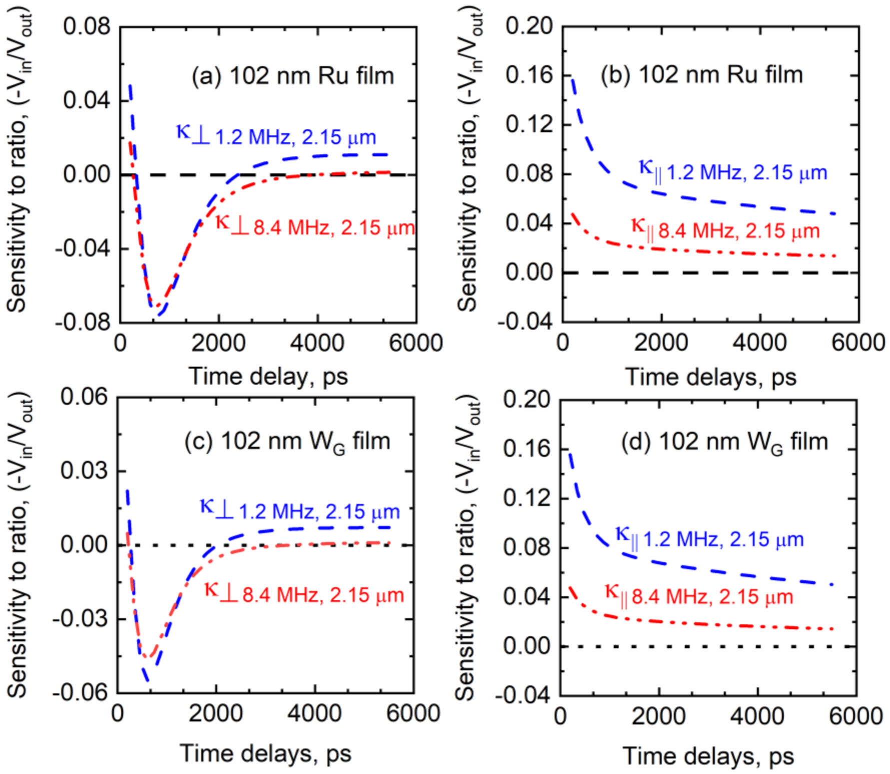


*Figure S17: TDTR measurement sensitivities to (a and c) the cross-plane thermal conductivity ($\kappa_{\perp}$) of Al/Ti coated 102 nm Ru and W films at different modulation frequencies and 2.15* µm *effective radii of beam. (b and d) The sensitivity to in-plane thermal conductivity* ($\kappa_{\parallel}$) *of these films.*

We determine the cross-plane and in-plane thermal conductivities of Ru and W films using a five-layer heat diffusion model.[25–27] Figure S18 shows how the best-fit thermal model aligns with the ratio of the in-phase and out-of-phase signals ($-V_{in}/V_{out}$), demonstrating the fitting process for both thermal conductivities. Table 1 (main manuscript) and Table S4 list the thermophysical properties and thicknesses of the individual layers used in the thermal model. We first measure the cross-plane thermal conductivity of Ru and W and then use it as an input parameter to extract the in-plane thermal conductivity. Table S4 presents the TDTR-measured values for cross-plane and in-plane thermal conductivities along with the thermal boundary resistance. Figure S19 displays the residual contours, comparing the model's fit to the best-fit values of cross-plane and in-plane thermal conductivities and the thermal boundary resistance at the Ti-film interface. The residual error between the theoretical model and experimental data reaches a maximum of approximately 1.5%, indicating that multiple combinations of thermal conductivity and boundary resistance can achieve a similar fit. Based on this, we set a 1.5% residual threshold, ensuring that the model consistently produces high-quality fits to the experimental data. The strong agreement within this threshold confirms that TDTR effectively detects variations in cross and in-plane thermal conductivities.

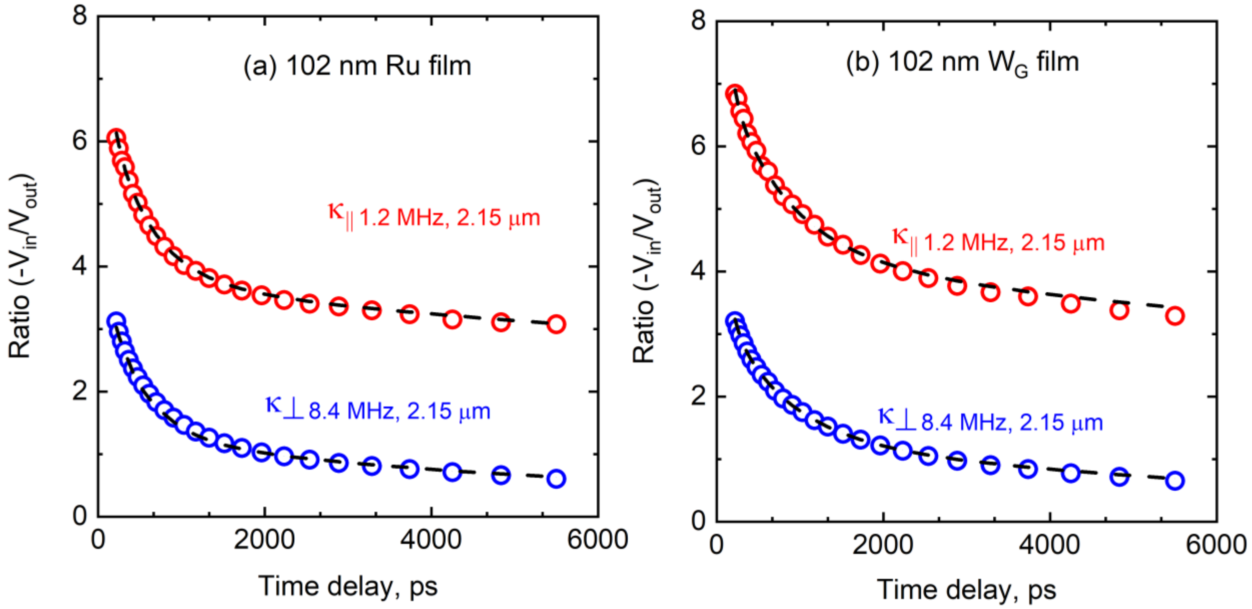


*Figure S18: Theoretical fit of experimental data for (a) annealed 102 nm Ru and (b) as-deposited 102 nm $W_G$ films.*

We incorporate the 1.5% residual uncertainty along with spot-to-spot variations in thermal conductivity, the thermal conductivities of Al, Ti, $SiO_2$, and Si, and the thermal boundary resistances into our total uncertainty ($\varepsilon_i$) calculation, as defined by the following equation:

Total uncertainty ($\varepsilon_i$),

$$\varepsilon_i = \sqrt{(\sigma_i{}^2) + \sum_i \Delta_i^2)} \qquad \text{(S06)}$$

Here $\sigma_i$ represents the standard deviations among multiple measurements taken different locations of the samples and $\Delta_i$ denotes the uncertainty associated with each individual parameter in the thermal model[21,28]. Table S4 presents the TDTR-measured thermal conductivities of Ru and W films, along with their corresponding thermal boundary resistances.

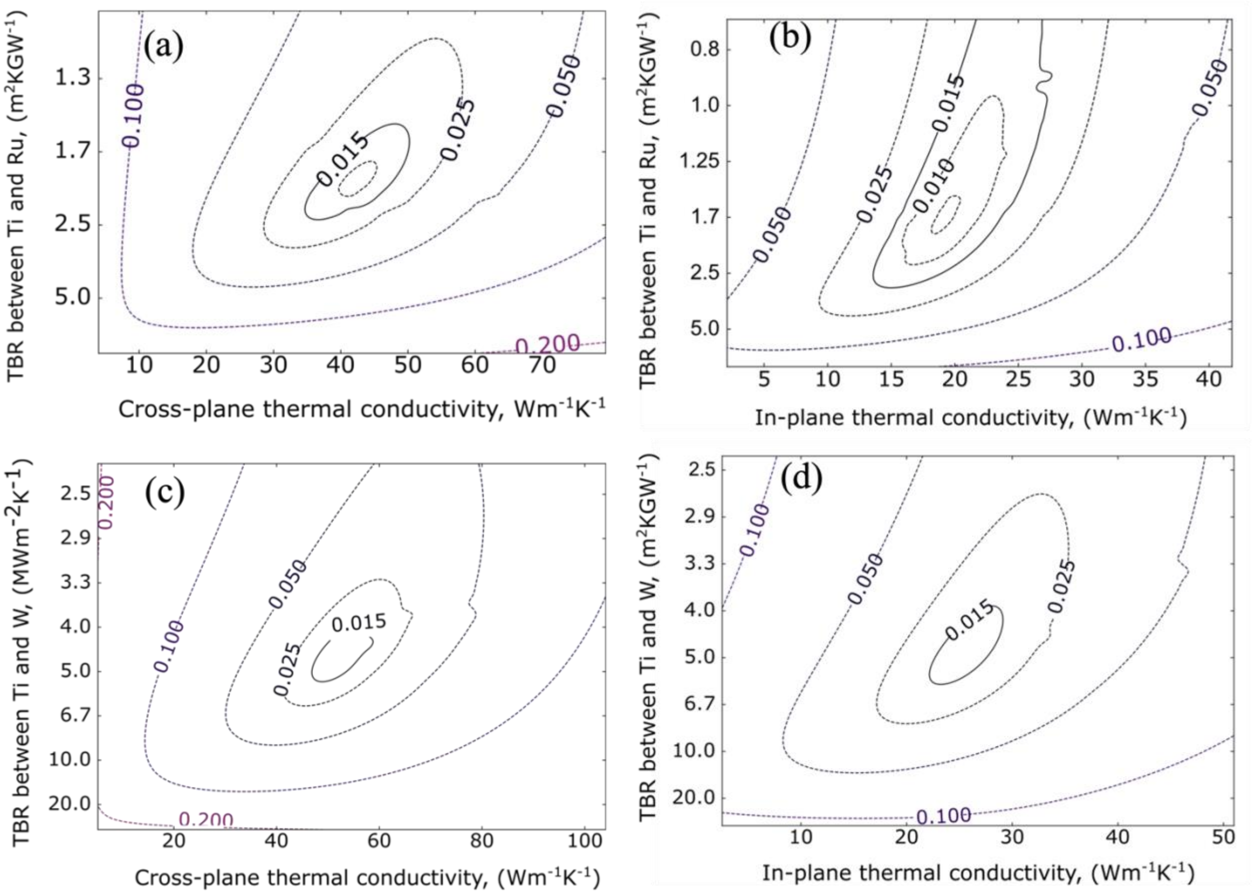


*Figure S19: Residual contours of our model's fit relative to the best fit for annealed 102 nm Ru and as-deposited 102 nm $W_G$ films as a function of cross and in-plane thermal conductivity. We choose 1.5% residual threshold within which the thermal model generates the same quality of fit to the experimental data.*

*Table S4: Parameters used in sensitivity analysis and the thermal model to determine the in-plane and cross-plane thermal conductivities of the Ru and W films.*

| Materials | Thickness, nm | Heat capacity, $MJm^{-3}K^{-1}$ | Thermal conductivity, $W\ m^{-1}\ K^{-1}$ | Thermal boundary resistance, (TBR) $m^2\ K\ GW^{-1}$ |
|---|---|---|---|---|
| Al | 20±1 | 2.42[20] | 110-120 | |
| Al/Ti | -- | -- | -- | 0.333[29–31] |
| Ti | 60±2 | 2.36[32] | 16-19 | |
| $Al_2O_3$ | | 3.06[32] | 34±1.5 [21,33] | |
| Ti/$Al_2O_3$ | -- | -- | -- | ~2.5-3.8 |
| Ti/Ru | -- | -- | -- | 0.86 (as-deposited)[a] |
| | | | | 1.52 (annealed)[a] |
| Ti/$W_G$ | -- | -- | -- | 4.52[a] |
| Ti/$W_R$ | -- | -- | -- | 1.00[29–31] |
| Ru | 5 -102 | 2.97[34] | As-deposited 102 nm, $\kappa_{\perp}$ =42.4±11.5 $Wm^{-1}K^{-1}$ | |
| | | | Annealed 102 nm, $\kappa_{\perp}$ =44.0±10.4 $Wm^{-1}K^{-1}$<br>$\kappa_{\parallel}$ = 21.3±11.2 $Wm^{-1}K^{-1}$ | |
| W | 3-102 | 2.56[35] | As-deposited 102 nm $W_G$, $\kappa_{\perp}$ = 52.8±12.4 $Wm^{-1}K^{-1}$<br>$\kappa_{\parallel}$ = 24.8±13.8 $Wm^{-1}K^{-1}$ | |
| Ru/$SiO_2$ and W/$SiO_2$ | | | | 5.00 [23] |
| $SiO_2$ | 100 | 1.62 [21–23] | 1.45[20,21,23,24] | |
| $SiO_2$/Si | - | - | - | 4.35 [22,23] |
| Si | - | 1.65[20–24] | 140 [21,23] | - |

a. We determine the in-plane thermal conductivity using SSTR, employing the TDTR best-fit values for cross-plane thermal conductivity and thermal boundary resistance (TBR) from 102 nm Ru. We assume that the TBR remains unchanged for the 32 nm and 52 nm Ru films. Similarly, for the 102 nm $W_G$ film, the TBR between Ti and $W_G$ is obtained from TDTR measurements and applied to 31 and 50 nm $W_G$ films. In contrast, the TBR between Ti and $W_R$ for 20–30 nm thick films is assumed to be 1 $m^2KGW^{-1}$ based on literature values and observations from this study. A 50% uncertainty is propagated for both measured and assumed TBR values.

b. We introduce perturbations in the thermal conductivity of Al, Ti, and Si by 5%, and that of $SiO_2$ by 3%. The measured TDTR cross-plane thermal conductivities of Ru and W is perturbed by 50%, as well as both measured and assumed thermal boundary resistances, are perturbed by 50%.

## S6. SSTR sensitivity, uncertainty and data analysis

To evaluate the sensitivity of SSTR measurements to the in-plane thermal conductivity of Ru and W films, we conduct a sensitivity analysis. We compute the SSTR sensitivities ($S_x$) to various thermal parameters in our samples as a function of Ru and W film thicknesses, employing a tightly focused laser spot. This analysis follows our prior methodology[1] and aligns with the approaches of Braun et al. and Yang et al. [21,36]

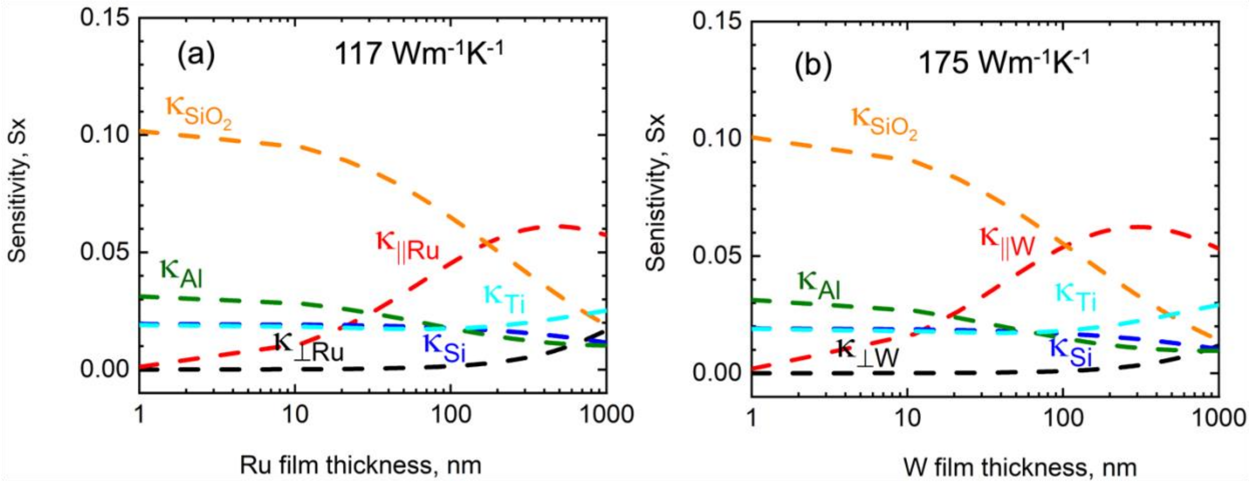


*Figure S20: (a) and (b) Typical sample stack of Ru and W films with an Al/Ti transducer as a function of film thickness. The analysis is performed at an effective radius ($\sqrt{r_0^2 + r_1^2}$) of 2.33 µm. The sensitivity to in-plane thermal conductivity ($\kappa_{\parallel}$) of Ru and W films is higher than its cross-plane thermal conductivity ($\kappa_{\perp}$) . SSTR maintains its sensitivity down to 30 nm Ru and 20 nm W films*

The sensitivity is determined using the following equation:

$$S_x = \frac{\Delta T_{1.1x}(thickness) - \Delta T_{0.9x}(thickness)}{\Delta T_x(thickness)} \qquad \text{(S07)}$$

Here $\Delta T_x$ is the temperature rise using the steady-state thermal model based on the given input parameters. In Equation S06, the input variables include x and the thicknesses of the Ru and W films, with values obtained from Table S4. Figure S20(a–b) shows that the sensitivity to in-plane thermal conductivity is greater than that to cross-plane conductivity. This occurs because Ru and W thin films have significantly higher thermal conductivity than $SiO_2$, causing heat to flow predominantly along the in-plane direction of the Ru and W films.[21,37] As a result, the in-plane temperature gradient is much steeper than the cross-plane gradient. Consequently, in-plane thermal conductivity primarily governs the sensitivity calculations in this study, allowing SSTR to effectively measure in-plane thermal conductivity. We determine the cross-plane thermal conductivity of Ru and W using TDTR (Table S4) and incorporate these values into the thermal model for SSTR analysis. In our SSTR system, we evaluate the sensitivity to in-plane thermal conductivity using an effective spot radius of ~2.33µm, which enhances lateral heat spreading.[1] We generate Figure S20(a-b) by assuming $\kappa_{\perp Ru} = \kappa_{\parallel Ru}$ = 117 W m$^{-1}$ K$^{-1}$ and $\kappa_{\perp W} = \kappa_{\parallel W}$ = 175

W $m^{-1}$ $K^{-1}$, respectively. However, Figure S20 also indicates that for film thickness up to ~100 nm, the sensitivity to the thermal conductivity of $SiO_2$ exceeds to in-plane thermal conductivity. To extract in-plane thermal conductivity of Ru and W, we use widely accepted value of $\kappa_{SiO2}$= 1.45 $Wm^{-1}K^{-1}$ [20,21,23,24] in our thermal model. Figure S20 further shows that the sensitivity to the thermal conductivity of Al and Ti is higher than that to the cross-plane thermal conductivity of Ru and W. Specifically, the sensitivity to Ti's thermal conductivity increases for film thicknesses beyond ~100 nm. We also use well-established literature values for the thermal conductivity of Si, as provided in Table S4. We obtain the heat capacity and thermal boundary resistances used in the sensitivity calculations from literature sources, as detailed in Table S4.[20–22,32]

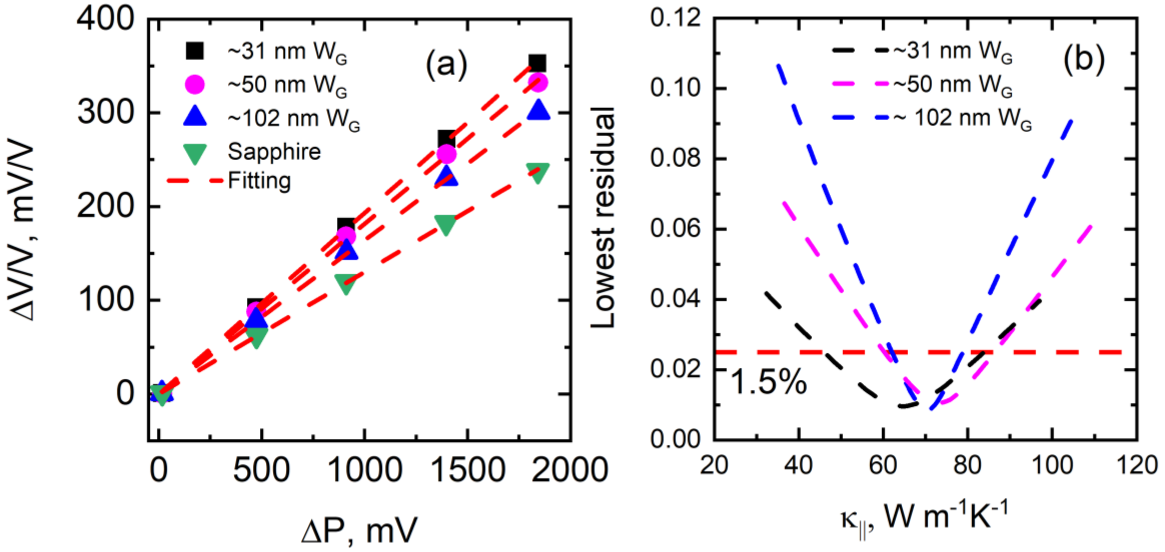


*Figure S21: (a) SSTR fitting of ΔV/V as a function of ΔP (proportional to pump power) to extract the thermal conductivities of sapphire and $W_G$ films, measured using an effective radius of ~ 2.33 µm. (b) Corresponding 2D contour analysis illustrating the quality of fit between the model parameters and experimental data, where the contour threshold is set to 1.5% based on the observed maximum residual error between the experimental and model data.*

SSTR measurements determine the in-plane thermal conductivity of Ru and W films by fitting, while other material properties come from TDTR or literature (Table S4). Figure S21a shows ΔV/V vs. ΔP, used in SSTR fitting to extract the thermal conductivities of sapphire and as-deposited $W_G$ films, following established procedures.[1,21] The calibration factor (γ) is derived from a sapphire reference sample with known transducer and sapphire properties (Table S4) and remains constant across samples. Using this calibration, we calculate the thermal conductivity of Al/Ti-coated $W_G$ films through a steady-state thermal model, applying a five-layer structure (Al/Ti transducer/$W_G$ thin film/$SiO_2$ /Si substrate) with properties listed in Table 1 and Table S4.

To account for the sensitivity of thermal parameters, we use contour plots to assess the similarity between experimental and model fits, identifying parameter interdependence while extracting the in-plane thermal conductivity of Ru and $W_G$. We compare measured SSTR data with a thermal model, iterating the in-plane thermal conductivity to achieve the best fit. Figure S21b demonstrates

a fit quality within a 1.5% residual, confirming SSTR's capability to measure in-plane thermal conductivity. We set the contour threshold to 1.5% based on the observed maximum residual error between the experimental and model data.[28,38] Error bars in the manuscript, calculated using Equation S4, account for residual uncertainty, spot-to-spot conductivity variations, and perturbations in layer conductivities and thermal boundary resistances (Table S4).

Table S5 compares the in-plane thermal conductivities measured by SSTR and TDTR. TDTR underpredicts thermal conductivity for these thin films due to its higher sensitivity to interface resistances within the film stacks. Unlike SSTR, TDTR accounts for interfacial resistances that cannot be separated during analysis, resulting in reduced measured values.[1,39] This reduction likely reflects an artifact of TDTR measurements, representing "effective" in-plane thermal conductivities of Ru and $W_G$, whereas SSTR provides values that more accurately reflect the intrinsic properties.

*Table S5: Comparison of SSTR, and TDTR measured in-plane thermal conductivities of Ru and W films.*

| *Film thickness, nm* | *TDTR, $Wm^{-1}K^{-1}$* | *SSTR, $Wm^{-1}K^{-1}$* |
|---|---|---|
| *Annealed ~102 nm Ru* | 21.3 ±11.2 | 75.1±9.9 |
| *As-deposited ~102 nm $W_G$* | 24.8±13.8 | *76.1±8.5* |

## S7: Beam offset technique

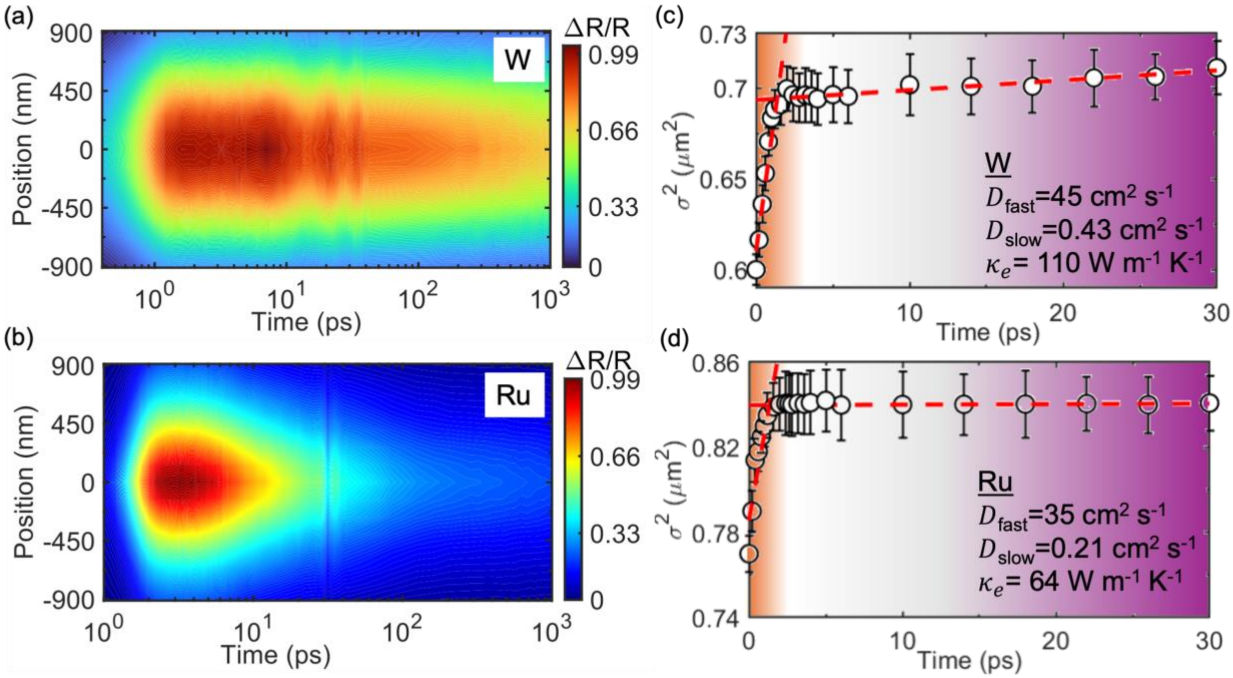


Figure S22: Contours showing the spatiotemporal profiles obtained with nanometric precision for (a) 30 nm W and (b) 100 nm Ru films. The square of the full-width at half maximum ($\sigma^2$) obtained from the gaussian profiles at various pump-probe time delays is plotted for (c) W and (d) Ru.

Figure S22 shows a typical beam-offset measurement on Ru and W. The details of our beam offset measurement can be found in the method section and somewhere else.[40] Figure S22a and S22b shows the electronic temperature dominates the spatiotemporal profile at early time delays while at later times, the profile is dictated by both electronic and phononic temperatures after they coupled with each other. From the spatiotemporal profile we obtain the gaussian profiles at different pump-probe time delays, which gives us an insight into the carrier diffusion processes. The square of the full-width at half maximum ($\sigma^2$) obtained from the gaussian profiles at various pump-probe time delays is plotted in Figure S22c and S22d. The fast diffusion regime at early times related to the equilibration of photo-excited electrons that couple with the cooler lattice leading to a steady slow diffusion regime in the later times after the coupling of electrons with the phonons. The slow diffusion regime is used to back out the thermal conductivity of the metallic films using the diffusivity equations.

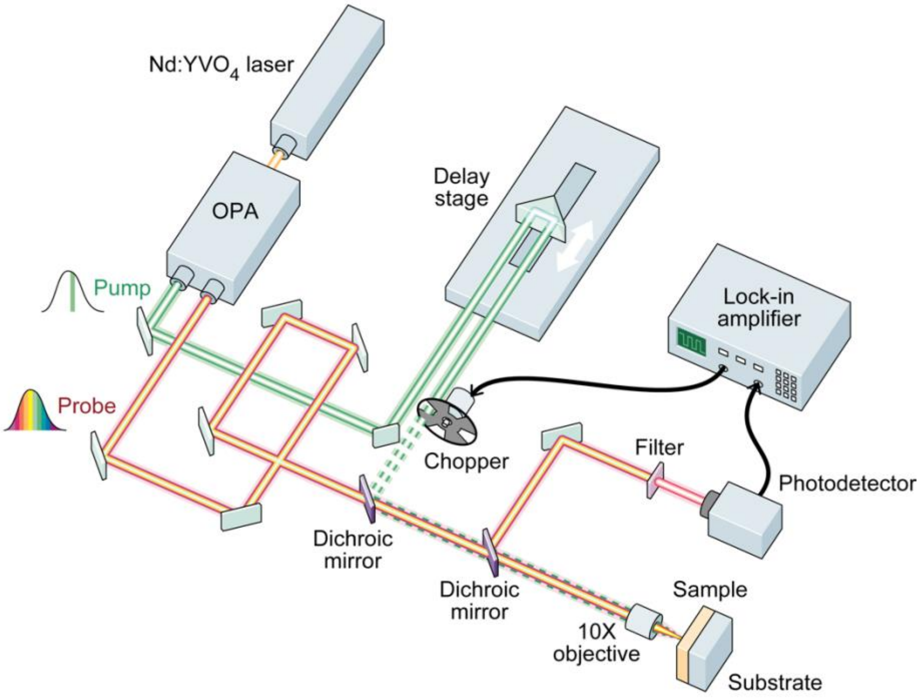


*Figure S23: Schematic of transient thermoreflectance pump-probe technique with infrared wavelength tunability.*

**S8. Details on two temperature model (TTM) and electron-phonon coupling factor determination.**

We use an ultrafast pump-probe technique with infrared wavelength tunability to study electron-phonon scattering in Ru and W films by monitoring their intraband transient thermoreflectance response. Figure S23 shows the experimental setup, where a Nd:$YVO_4$ laser (~1040 nm, 1 MHz) passes through an OPA, generating a 520 nm pump beam via SHG and a tunable probe (600–2500 nm). We chop the 379 fs pump pulses at 450 Hz and measure their duration by fitting Pt thermoreflectance signals using a *sech²* function.[1] In this experiment, we excite electrons in Ru

and W films with a 2.38 eV pump, driving them out of equilibrium with phonons. We then probe the thermoreflectance at ~0.53 eV (Ru) and ~0.56 eV (W), ensuring a nearly free-electron-like reflectivity response by choosing probe energies far from the interband transition thresholds [Ru: 1.74 ± 0.02 eV; W: 0.94 ± 0.05, 1.80 ± 0.015 eV] determined via our ellipsometer (see in the following section). This approach simplifies the extraction of the electron–phonon coupling factor ($G$) of the films[41], as the thermoreflectance signal remains linearly proportional to the phonon subsystem temperature,[42,43] while the electron subsystem's contribution is negligible. We perform measurements at low pump power (fluence ≈ 8.42 J/m²) to prevent nonlinear thermophysical effects,[44] maintaining a linear relationship between electron temperature and material properties ($\Delta T_e \approx 708.8$ K). Figure S24 presents the thermoreflectance response of Ru and W films, showing that free electrons transfer energy to phonons within a sub-picosecond timescale. The rise time of the reflectance signals in as-deposited Ru and W films, regardless of thickness and grain size, remains constant, indicating that these factors do not influence electron-phonon energy transfer. However, Figure S25 shows that the thermoreflectance behavior differs between Ru and W films. The rise time in W films is slower within the time regime relevant to electron-phonon interactions compared to that of Ru, suggesting that the electron-phonon coupling factor in Ru is higher than that in W.

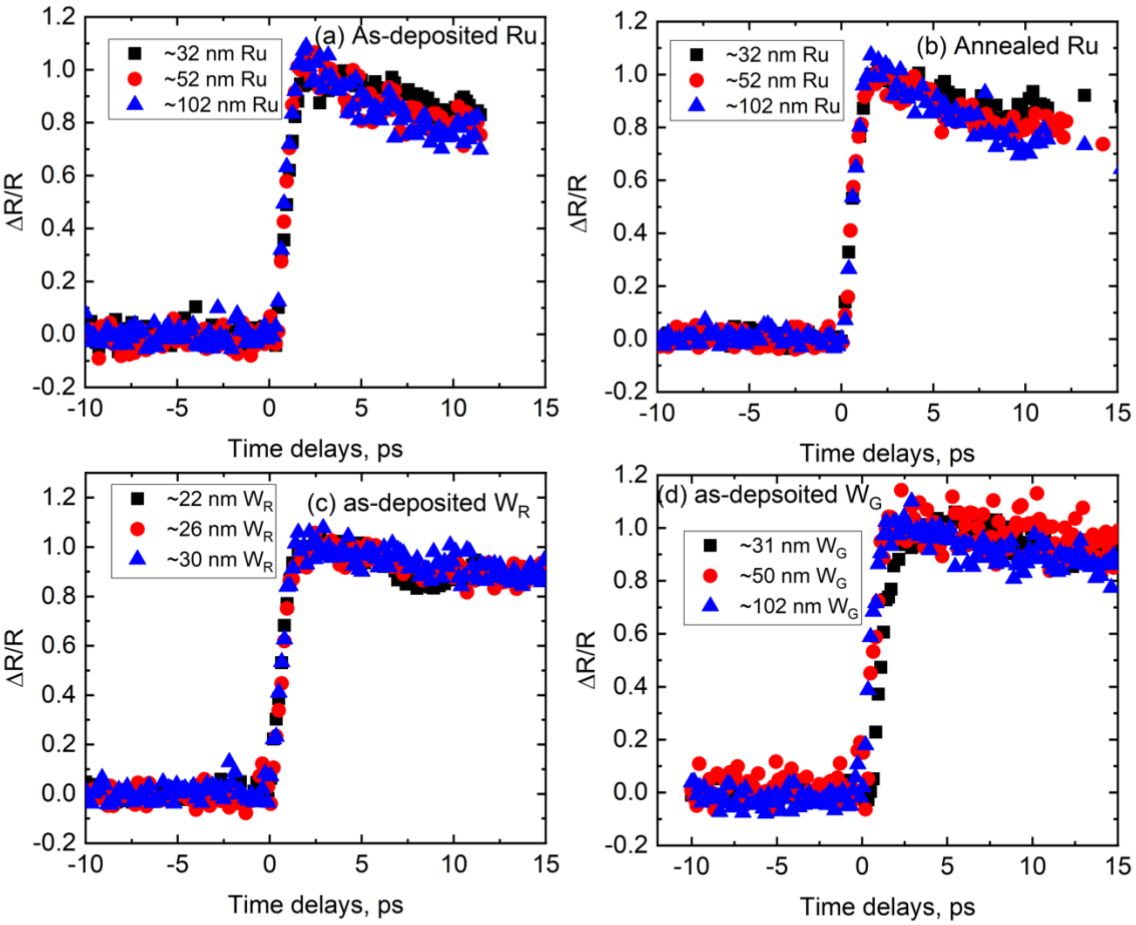

*Figure S24: Normalized thermoreflectance as a function of pump-probe delay time for as-deposited Ru and W films.*

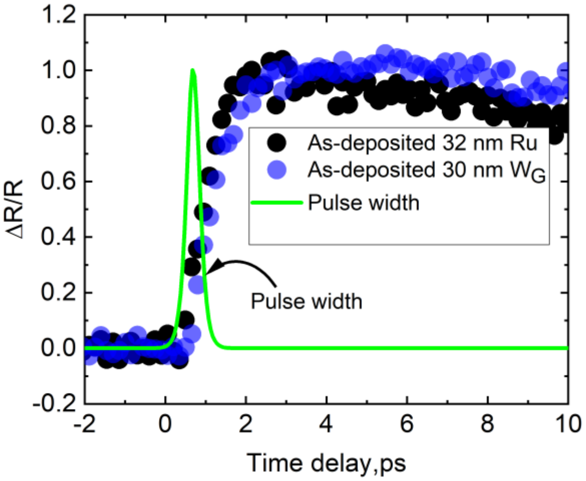


*Figure S25: The comparison of the normalized thermoreflectance as a function of pump-probe delay time for as-deposited Ru and W films.*

We apply the two-temperature model (TTM) to determine the electron-phonon coupling factors in Ru and W films using the following equations:

$$C_e(T_e)\frac{\partial T_e}{\partial t} = \nabla \cdot (\kappa_e \nabla T_e) - G(T_e - T_p) + S(x,t) \qquad (S08)$$

$$C_p(T_p)\frac{\partial T_p}{\partial t} = \nabla \cdot (\kappa_p \nabla T_p) + G(T_e - T_p) \qquad (\mathrm{S09})$$

Here, $C_e$ and $C_p$ represents the heat capacities of the electrons and phonons, respectively, while $T_e$ and $T_p$ denote their temperatures. The source term, S (x, t) is given by[45] :

$$S(x,t) = (1 - R_{opt})\frac{1.76J}{2t_p} \cdot sech^2\left[\left(\frac{1.76(t_o - t)}{t_p}\right)\right]\frac{dI}{dx} \qquad (\mathrm{S10})$$

In this equation, $R_{opt}$ denotes the surface reflectivity, $J$ is the incident fluence, $t_p$ is pulse width of the pump pulse, $\frac{dI}{dx}$ is the light intensity profile determined using a transfer matrix method based on optical constants at the 520 nm pump wavelength. This profile is computed following the Beer–Lambert law and assumes a $sech^2$ pulse shape in the time domain.

We employ the Crank-Nicolson method[46] to solve the coupled differential equations in the two-temperature model (TTM) and determine the electron-phonon coupling factor. To ensure numerical stability, we discretize time ($dt = 50 \times 10^{-15}$ s) and space ($dx = 0.5 \times 10^{-9}$ m) based on the material parameters listed in Table S6. Using the transfer matrix method, [47] we calculate the light intensity distribution in the Ru/100 nm $SiO_2$/Si and W/3nm Ta/100 nm $SiO_2$/Si systems and model energy deposition into the electronic system through the source term S. We assume the 3 nm Ta layer as the interface between W and 100 nm $SiO_2$. For films ≤30 nm, we neglect the thermal conductivity terms in the TTM equations (Eq. S08 and Eq. S09) because the film heats homogeneously on timescales relevant to electron-phonon coupling. The optical penetration depth

of the pump beam (7.7 ± 0.04 nm for Ru and 13.1 ± 0.3 nm for W) determined via the ellipsometer (see details in the following section) is smaller than 30 nm, ensuring that energy deposition primarily occurs near the surface. However, rapid electron scattering, with mean free paths of 6 nm for Ru[4,48] and 15.5 nm for W[4,48], facilitates energy redistribution across the film thickness before significant phonon interactions occur. Additionally, ballistic electron transport further enhances energy spreading, allowing the electrons to rapidly thermalize within the film thickness before phonon-driven heat dissipation dominates. For ~50 nm and ~100 nm films, we incorporate the thermal conductivity terms in TTM to determine G, as heat conduction effects become more significant over longer distances. We also assume that the electronic heat capacity varies linearly with electron temperature and that the electron-phonon coupling factor remains constant with temperature.

We use TTM simulations to calculate the lattice and electron temperatures based on the thermophysical properties listed in Table S6. Since our probing energy is well above interband transition thresholds, we convert the TTM simulation results into an optical response by normalizing the lattice temperature and comparing it to the normalized reflectivity from thermoreflectance measurements. We normalize the data using the average value of ΔR/R between 1–3 ps and fit for *G* within the 0–10 ps range. This time window allows sufficient electron-phonon coupling and ensures the lattice temperature reaches its peak (Figure S26)

*Table S6: We list the parameters used for the TTM calculations. The temperature-dependent coefficient of the electronic heat capacity,* $\beta$*,* $(Ce = \beta T_e)$*, is obtained from our first-principles simulations ( see Section S2) which show good agreement well with the literature,* $(C_e = \beta T_e)$*,* $C_p$ *denotes the phonon heat capacity, while* $\kappa_e$*and* $\kappa_p$ *represent the thermal conductivity of the electron and phonon subsystems, respectively. These thermal conductivities are determined from 4-pp measurements and SSTR. The electronic thermal boundary resistance is negligible, while the phononic thermal boundary resistances used in the TTM simulations are Ru/*$SiO_2$*= 5* $m^2$ *K* $GW^{-1}$ *[23] ,W/*$SiO_2$*=5* $m^2$ *K* $GW^{-1}$ *[23],* $SiO_2$*/Si=4.35* $m^2$ *K* $GW^{-1}$ *[22,23] .*

| Parameters | Ru | W | $SiO_2$ | Si |
|---|---|---|---|---|
| Electron heat capacity coefficient, $\beta$ (J $m^{-3}$ $K^{-2}$) | 371 | 137.3 | 0 | 0 |
| Electron thermal conductivity, $\kappa_e$ (W $m^{-1}$ $k^{-1}$) | 29-52 | 35-40 | 0 | 0 |
| Phonon thermal conductivity, $\kappa_p$ (W $m^{-1}$ $k^{-1}$) | 25-32 | 30-64 | 1.45 [20,21,23,24] | 140 [21,23] |
| Phonon heat capacity, $C_p$ (MJ $m^{-3}K^{-1}$) | 2.85 | 2.52 | 1.62[21–23] | 1.65[20–24] |

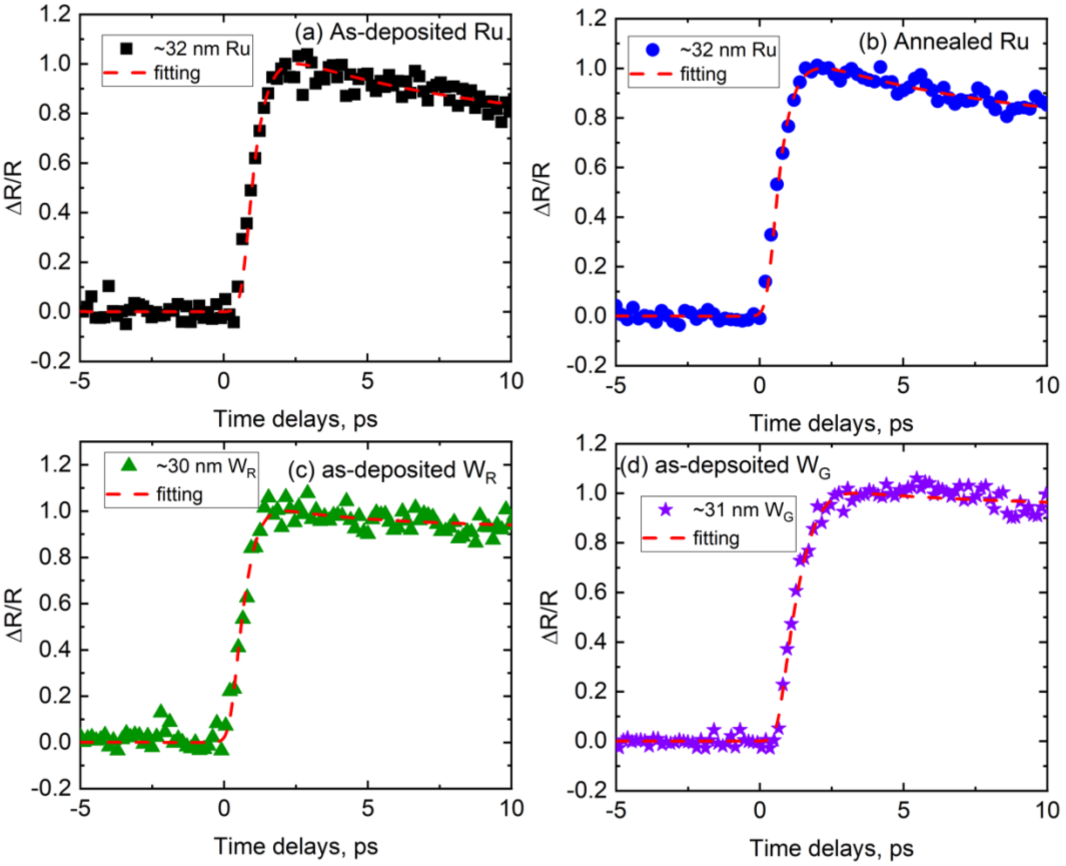


*Figure S26: Experimental data for as-deposited Ru and W films. The orange dashed line is the best fit to experimental data.*

During the electron-phonon coupling factor (G) analysis, we assess whether the fitting parameters in the TTM exhibit sufficient sensitivity to determine G accurately. While the characteristic response within the 0–10 ps time regime primarily arises from electron-phonon coupling, variations in G exist for Ru and W films due to experimental noise, leading to multiple acceptable fits to the data. To quantify this uncertainty, we employ contour plots that evaluate the similarity between different fits of the experimental and model data. We generate the optical response curve using TTM with the best-fit set of material properties (Table S6) and perturb G by re-fitting. In this process, we fit only for the time at which the pulse interacts with the sample: an arbitrary parameter in our TTM. The degree of similarity between the perturbed curve and the experimental data, relative to the best-fit curve, establishes the uncertainty bounds. To quantify this, we apply the metric defined by Feser et al.:[28]

$$Z(G) \equiv \left(\frac{\sum[reflectivity(t;G_{exact})-reflectivity(t;G_{perturbed})]^{2}}{\sum reflectivity(t;G_{exact})^{2}}\right)^{\frac{1}{2}} \qquad \text{(S11)}$$

The contour of Z(G) characterizes the least-squares similarity between different fits, where the curvature around the best-fit value (global minimum) defines the uncertainty. Based on the quality of our experimental data, we adopt a 0.5% residual threshold, within which the TTM produces fits of comparable quality to the experimental data, as illustrated in Figure S27. We incorporate this 0.5% residual uncertainty into the overall uncertainty in our G calculations.

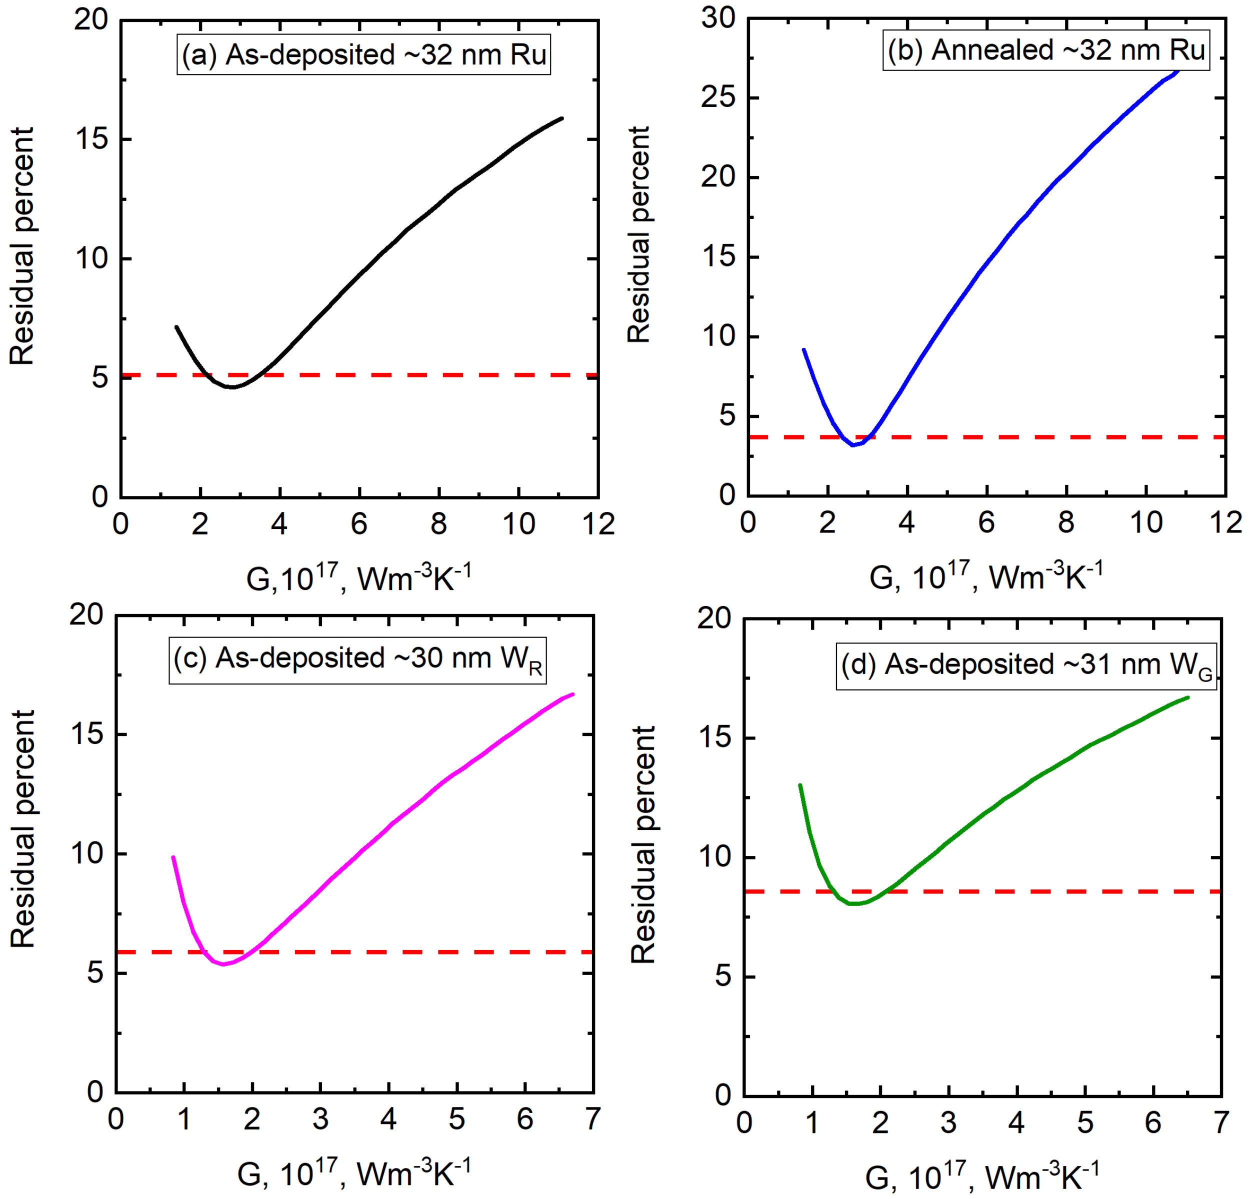


*Figure S27: 2D contour analysis of G for as-deposited Cu films assuming the quality of fit based on the TTM model parameters and experimental data is within 0.5% threshold value.*

## S09. Effective electron relaxation time, interband transitions and optical penetration depth determination with ellipsometer

We determine the optical penetration depth of Ru and W using a visible ellipsometer (M2000, J.A. Woollam Company) at a wavelength of 520 nm (2.3842 eV). Figure S28 presents the optical response of Ru films of varying thicknesses, characterized by their dielectric functions ($\varepsilon_1$ and $\varepsilon_2$).

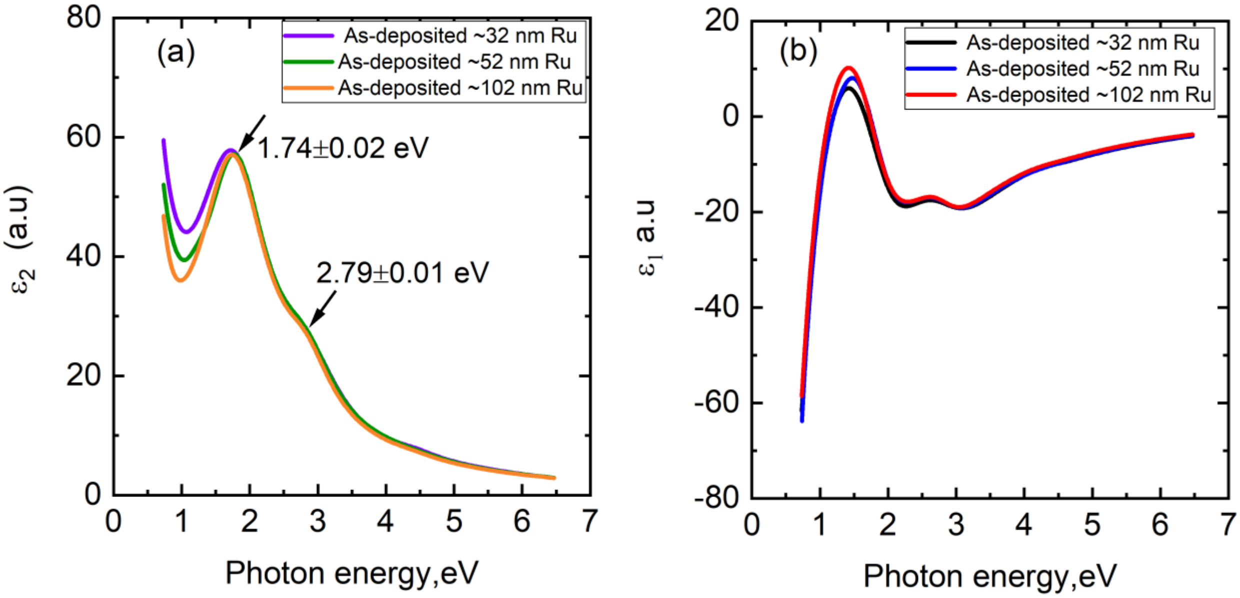


*Figure S28: The optical response of as-deposited Ru films as a function of photon energy (0.73eV-6.53eV). The interband transitions in Ru happen at* 1.74±0.02 eV and 2.79± 0.01 eV. No interband transitions are observed below ~0.73 eV photon energy.

Figure S28 shows the optical response of different thick Ru films in terms of dielectric functions ($\varepsilon_1$ and $\varepsilon_2$ ). We identify the interband transition for Ru at 1.74±0.02 eV and 2.79± 0.01 eV. Similarly for the W, the interband transitions occur at 0.94 ± 0.05 and 1.80 ± 0.015 eV. The optical penetration depths for Ru and W are calculated as 7.7 ± 0.04 nm and 13.1 ± 0.3 nm, respectively, using following relation, penetration depth: $\delta = \frac{\lambda}{4\pi\sqrt{Im(\epsilon)}}$ (S12)

where λ is the incident light wavelength, and Im(ε) represents the imaginary part of the dielectric function, which incorporates the material's absorption coefficient.

We use infrared variable-angle spectroscopic ellipsometry (IR-VASE) to determine the effective electron relaxation time in materials by analyzing their optical properties in the infrared spectrum. By fitting oscillator models to complex, frequency-dependent ellipsometric data, we extract the effective electron relaxation time for Ru and W films. Ellipsometry measures the change in polarization state of the light upon reflection from the sample, capturing the amplitude ratio (Ψ) and phase difference (Δ). These parameters relate to the complex reflection coefficients ($r_p$ and $r_s$) of the sample for $p$- and $s$-polarized light as:

$$\rho = \frac{r_p}{r_s} = \tan\Psi\, e^{i\Delta} \qquad \text{(S13)}$$

We collect ellipsometric data for Ru and W films over the spectral range of 500-3500 cm$^{-1}$ (0.06-0.433 eV) using an infrared ellipsometer (IR-VASE Mark II, J.A. Woollam Company). We perform the measurements at ncident angles of 60° and 70°, with a spectral resolution of 16 cm$^{-1}$ (~2 meV). Figure S29 presents the measured ellipsometric data for as-deposited Ru films with thicknesses ranging from 5 nm to 102 nm.

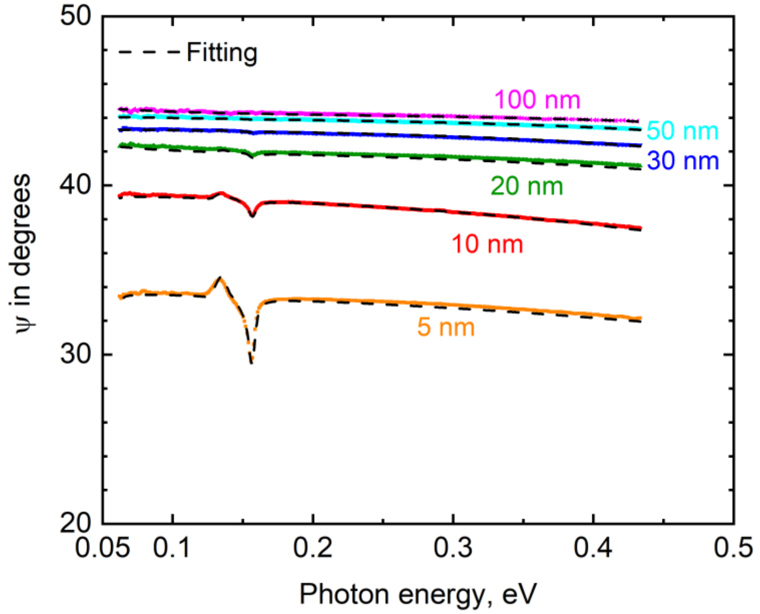


*Figure S29: (a) Measured ellipsometry data at the incidence angle of 60° for as-deposited Ru films with various thicknesses and their comparison of measured ellipsometry data for with modeling results (black lines) fitted on the measured data.*

We develop an isotropic multi-layer optical model based on this measured ellipsometric data to extract the complex, frequency-dependent dielectric function of the Ru and W film. For the dielectric functions of the silicon substrate and thermal $SiO_2$ layer,[49] we use literature-reported values. In the infrared regime, the optical properties of the Ru and W films are primarily dominated by the free-electron contribution. Therefore, we apply the Drude-Lorentz model to determine the optical behavior as follows: [50]

$$\varepsilon_{Drude-Lorentz}(\omega) = \varepsilon_1(\omega) + i\varepsilon_2(\omega) = \varepsilon_\infty - \frac{\omega_p^2}{\omega^2 + i\Gamma\omega} + \sum_i \frac{f_i}{\omega_i^2 - \omega^2 - i\Gamma_i\omega} \quad \text{(S14)}$$

In this expression, $\varepsilon_\infty$ is the high-frequency dielectric constant, the second term on the right side describes free-electron contribution[50] where $\omega_p$ is the plasma frequency, and $\Gamma$ is the scattering rate. The third term on the right side describes the effect of electronic transition modes to the near-

infrared excited response. These transitions are modeled using the Lorentz function[50], where $f_i$ is the oscillator strength, $\omega_i$ the resonance frequency, and $\Gamma i$ the broadening parameter of the i-th oscillator.

We refine the parameters of the Drude-Lorentz model by minimizing the mean square error to achieve optimal agreement between the modeled and measured ellipsometric data. Figure S29 presents a comparison between the fitted modeling results and the measured data for two representative as-deposited Ru films at the incidence angle of 60°. The mean squared errors for the fits across different film thicknesses remain 0.3, indicating a high level of accuracy. Finally, we determine the effective relaxation time of electron ($\tau$) from the fitted scattering rate in the Drude model, where $\tau = \Gamma^{-1}$.

Reference


1. Islam, M. R. *et al.* Evaluating size effects on the thermal conductivity and electron-phonon scattering rates of copper thin films for experimental validation of Matthiessen's rule. *Nat Commun* **15**, 9167 (2024).
2. Karna, P. & Giri, A. Effect of intense laser irradiation on the thermal transport properties of metals. *Phys. Rev. B* **107**, 094301 (2023).
3. Karna, P. & Giri, A. Electron–electron scattering limits thermal conductivity of metals under extremely high electron temperatures. *J. Phys.: Condens. Matter* **36**, 345701 (2024).
4. Karna, P., Islam, M. R., Hoglund, E. R., Hopkins, P. E. & Giri, A. Electron-phonon coupling dictates electron mean free paths and negative thermal diffusion in metals. *Materials Today Chemistry* **37**, 101991 (2024).
5. Hopkins, P. E., Serrano, J. R., Phinney, L. M., Li, H. & Misra, A. Boundary scattering effects during electron thermalization in nanoporous gold. *Journal of Applied Physics* **109**, 13524 (2011).
6. Klemens, P. G. The Scattering of Low-Frequency Lattice Waves by Static Imperfections. *Proc. Phys. Soc. A* **68**, 1113 (1955).

7. Lu, I.-T. & Bernardi, M. Using defects to store energy in materials – a computational study. *Sci Rep* **7**, 3403 (2017).

8. Nakagawa, M., Mansel, W., Böning, K., Rosner, P. & Vogl, G. Spontaneous recombination volumes of Frenkel defects in neutron-irradiated non-fcc metals. *Phys. Rev. B* **19**, 742–748 (1979).

9. Giannozzi, P. *et al.* QUANTUM ESPRESSO: a modular and open-source software project for quantum simulations of materials. *J. Phys.: Condens. Matter* **21**, 395502 (2009).

10. Martoňák, R., Laio, A. & Parrinello, M. Predicting Crystal Structures: The Parrinello-Rahman Method Revisited. *Phys. Rev. Lett.* **90**, 075503 (2003).

11. Developers, T. TensorFlow. *Zenodo* (2021) doi:10.5281/zenodo.4758419.

12. Thompson, A. P. *et al.* LAMMPS - a flexible simulation tool for particle-based materials modeling at the atomic, meso, and continuum scales. *Computer Physics Communications* **271**, 108171 (2022).

13. He, K., Zhang, X., Ren, S. & Sun, J. Deep Residual Learning for Image Recognition. in 770–778 (2016).

14. Thomas, J. A., Turney, J. E., Iutzi, R. M., Amon, C. H. & McGaughey, A. J. H. Predicting phonon dispersion relations and lifetimes from the spectral energy density. *Phys. Rev. B* **81**, 081411 (2010).

15. Feng, T., Qiu, B. & Ruan, X. Anharmonicity and necessity of phonon eigenvectors in the phonon normal mode analysis. *Journal of Applied Physics* **117**, 195102 (2015).

16. Hoover, W. G. Canonical dynamics: Equilibrium phase-space distributions. *Phys. Rev. A* **31**, 1695–1697 (1985).

17. Callaway, J. Model for Lattice Thermal Conductivity at Low Temperatures. *Phys. Rev.* **113**, 1046–1051 (1959).

18. Hirt, D. *et al.* Increased thermal conductivity and decreased electron–phonon coupling factor of the aluminum scandium intermetallic phase (Al3Sc) compared to solid solutions. *Applied Physics Letters* **124**, 202202 (2024).

19. Schmidt, A. J., Cheaito, R. & Chiesa, M. A frequency-domain thermoreflectance method for the characterization of thermal properties. *Review of Scientific Instruments* **80**, 94901 (2009).

20. Cancellieri, C. *et al.* Interface and layer periodicity effects on the thermal conductivity of copper-based nanomultilayers with tungsten, tantalum, and tantalum nitride diffusion barriers. *Journal of Applied Physics* **128**, (2020).

21. Braun, J. L., Olson, D. H., Gaskins, J. T. & Hopkins, P. E. A steady-state thermoreflectance method to measure thermal conductivity. *Review of Scientific Instruments* **90**, 24905 (2019).

22. Braun, J. L. *et al.* Size effects on the thermal conductivity of amorphous silicon thin films. *Physical Review B* **93**, 140201 (2016).

23. Hoque, M. S. B. *et al.* Thermal conductivity measurements of sub-surface buried substrates by steady-state thermoreflectance. *Review of Scientific Instruments* **92**, 64906 (2021).

24. Scott, E. A. *et al.* Thermal resistance and heat capacity in hafnium zirconium oxide (Hf1-xZrxO2) dielectrics and ferroelectric thin films. *Applied Physics Letters* **113**, 192901 (2018).

25. Cahill, D. G., Goodson, K. & Majumdar, A. Thermometry and Thermal Transport in Micro/Nanoscale Solid-State Devices and Structures. *Journal of Heat Transfer* **124**, 223–241 (2002).

26. Hopkins, P. E. *et al.* Criteria for cross-plane dominated thermal transport in multilayer thin film systems during modulated laser heating. *Journal of Heat Transfer* **132**, 1–10 (2010).

27. Cahill, D. G. Analysis of heat flow in layered structures for time-domain thermoreflectance. *Review of Scientific Instruments* **75**, 5119–5122 (2004).

28. Feser, J. P. & Cahill, D. G. Probing anisotropic heat transport using time-domain thermoreflectance with offset laser spots. *Review of Scientific Instruments* **83**, 104901 (2012).

29. Wilson, R. B. & Cahill, D. G. Experimental Validation of the Interfacial Form of the Wiedemann-Franz Law. 255901–255902 (2012) doi:10.1103/PhysRevLett.108.255901.

30. Cheaito, R. *et al.* Thermal flux limited electron Kapitza conductance in copper-niobium multilayers. *Applied Physics Letters* **106**, 93114 (2015).

31. Gundrum, B. C., Cahill, D. G. & Averback, R. S. Thermal conductance of metal-metal interfaces. doi:10.1103/PhysRevB.72.245426.

32. Olson, D. H. *et al.* Band alignment and defects influence the electron-phonon heat transport mechanisms across metal interfaces. *Applied Physics Letters* **118**, 163503 (2021).

33. Wilson, R. B. & Cahill, D. G. Limits to Fourier theory in high thermal conductivity single crystals . *Appl. Phys. Lett* **107**, 203112 (2015).

34. Jang, H., Kimling, J. & Cahill, D. G. Nonequilibrium heat transport in Pt and Ru probed by an ultrathin Co thermometer. *Phys. Rev. B* **101**, 064304 (2020).

35. Bodryakov, V. Yu. Correlation of temperature dependences of thermal expansion and heat capacity of refractory metal up to the melting point: Tungsten. *High Temp* **53**, 643–648 (2015).

36. Yang, J., Maragliano, C. & Schmidt, A. J. Thermal property microscopy with frequency domain thermoreflectance. *Review of Scientific Instruments* **84**, 104904 (2013).

37. Hoque, M. S. B. *et al.* High In-Plane Thermal Conductivity of Aluminum Nitride Thin Films. *ACS Nano* **15**, 9588–9599 (2021).

38. Pfeifer, T. W. *et al.* Measuring sub-surface spatially varying thermal conductivity of silicon implanted with krypton. *Journal of Applied Physics* **132**, (2022).

39. Zeng, T. & Chen, G. Phonon Heat Conduction in Thin Films: Impacts of Thermal Boundary Resistance and Internal Heat Generation. *Journal of Heat Transfer* **123**, 340–347 (2001).

40. Karna, P., Hoque, M. S. B., Thakur, S., Hopkins, P. E. & Giri, A. Direct Measurement of Ballistic and Diffusive Electron Transport in Gold. *Nano Lett.* **23**, 491–496 (2023).

41. Tomko, J. A., Kumar, S., Sundararaman, R. & Hopkins, P. E. Temperature dependent electron-phonon coupling of Au resolved via lattice dynamics measured with sub-picosecond infrared pulses. *Journal of Applied Physics* **129**, 193104 (2021).

42. Heilpern, T. *et al.* Determination of hot carrier energy distributions from inversion of ultrafast pump-probe reflectivity measurements. *Nature Communications 2018 9:1* **9**, 1–6 (2018).

43. Schoenlein, R. W., Lin, W. Z., Fujimoto, J. G. & Eesley, G. L. Femtosecond studies of nonequilibrium electronic processes in metals. *Physical Review Letters* **58**, 1680 (1987).

44. Lin, Z., Zhigilei, L. V. & Celli, V. Electron-phonon coupling and electron heat capacity of metals under conditions of strong electron-phonon nonequilibrium. *Physical Review B - Condensed Matter and Materials Physics* **77**, 075133 (2008).

45. Sotrop, J., Kersch, A., Domke, M., Heise, G. & Huber, H. P. Numerical simulation of ultrafast expansion as the driving mechanism for confined laser ablation with ultra-short laser pulses. *Applied Physics A: Materials Science and Processing* **113**, 397–411 (2013).

46. Özışık, M. N., Colaco, M. J., Orlande, H. R. B. & Cotta, R. M. *Finite Difference Methods in Heat Transfer*. (Taylor & Francis, CRC Press, 2017).

47. Bhatia, A. B. *et al.* Principles of optics Electromagnetic theory of propagation, interference and diffraction of light with contributions by SEVENTH HEXPANDED) EDITION.

48. Gall, D. Electron mean free path in elemental metals. *Journal of Applied Physics* **119**, (2016).

49. Herzinger, C. M., Johs, B., McGahan, W. A., Woollam, J. A. & Paulson, W. Ellipsometric determination of optical constants for silicon and thermally grown silicon dioxide via a multi-sample, multi-wavelength, multi-angle investigation. *Journal of Applied Physics* **83**, 3323–3336 (1998).

50. Fowles, G. R. *Introduction to Modern Optics*. (1989).
